# Supplementary material for: On 3-nondegenerate CR manifolds in dimension 7 (II): the intransitive case
Source: arXiv:2308.02841 ancillary file (2025-09-15)
Supplement: Supplementary file 1 [file 7D3ndg_II1.pdf]

Maple accompanying the paper "On 3-nondegenerate CR manifolds in dimension 7 (II): the intransitive case" by Boris Kruglikov and Andrea Santi.

>

This worksheet is devoted to computing the Jacobi relation ideal to exclude possible filtered deformations of higher dimensional candidates for symmetry with 6D orbit.

Note that even though the ideal is quadratic, it contains some linear generators, which we can resolve, then substitute and find new linear generators, and so forth.

Thus resolving the ideal does not involve any hard polynomial technique, and the condition that the ideal contains 1 (and hence its locus is vacuous) is mathematically rigorous.

>

We start by computing the Tanaka prolongation of the 6D orbit on 3ndg 7D CR of type  $\dim(U_L)=2$ ,  $\dim(U_K)=3$ , with 2D structure reduction.

> *restart* : *with* ( *DifferentialGeometry* ) : *with* ( *LieAlgebras* ) : *with* ( *GroupActions* ) : *with* ( *Tools* ) : *Preferences* ( "ShowFramePrompt", 'false' ) :

> *L* := *LieAlgebraData* ( [ [ *X10*, *X01* ] = *R* ], [ *R*, *X10*, *X01*, *Y*, *Z10*, *Z01* ], *alg*, *grading* = [ -2, -1, -1, -1, -1 ] ) :

> *DGsetup* ( *L* ) :

> *infolevel* [ *TanakaProlongation* ] := 2 :

> *prL0* := *TanakaProlongation* ( *alg*, 1, *pralg0* )

m:

[*e1*], [*e2*, *e3*, *e4*, *e5*, *e6*]  
[-2, -1]

$g^{(0)}$ :

[*e1*], [*e2*, *e3*, *e4*, *e5*, *e6*], [*e7*, *e8*, *e9*, *e10*, *e11*, *e12*, *e13*,  
*e14*, *e15*, *e16*, *e17*, *e18*, *e19*, *e20*, *e21*, *e22*, *e23*, *e24*, *e25*]  
[-2, -1, 0]

*prL0* := [ [*e1*, *e7*] = -*e1*, [*e2*, *e3*] = *e1*, [*e2*, *e8*] = -*e2*, [*e2*, *e10*] = -*e3*, [*e2*, *e11*] = -*e4*, [*e2*, *e16*] = -*e5*, [*e2*, *e21*] = -*e6*, [*e3*, *e7*] = -*e3*, [*e3*, *e8*] = *e3*, [*e3*, *e9*] = -*e2*, [*e3*, *e12*] = -*e4*, [*e3*, *e17*] = -*e5*, [*e3*, *e22*] = -*e6*, [*e4*, *e13*] = -*e4*, [*e4*, *e18*] = -*e5*, [*e4*, *e23*] = -*e6*, [*e5*, *e14*] = -*e4*, [*e5*, *e19*] = -*e5*, [*e5*, *e24*] = -*e6*, [*e6*, *e15*] = -*e4*, [*e6*, *e20*] = -*e5*, [*e6*, *e25*] = -*e6*, [*e7*, *e9*] = -*e9*, [*e7*, *e10*] = *e10*, [*e7*, *e12*] = -*e12*, [*e7*, *e17*] = -*e17*, [*e7*, *e22*] = -*e22*, [*e8*, *e9*] = 2 *e9*, [*e8*, *e10*] = -2 *e10*, [*e8*, *e11*] = -*e11*, [*e8*, *e12*] = *e12*, [*e8*, *e16*] = -*e16*, [*e8*, *e17*] = *e17*, [*e8*, *e21*] = -*e21*, [*e8*, *e22*] = *e22*, [*e9*, *e10*] = *e8*, [*e9*, *e11*] = -*e12*, [*e9*, *e16*] = -*e17*, [*e9*, *e21*] = -*e22*, [*e10*, *e12*] = -*e11*, [*e10*, *e17*] = -*e16*, [*e10*, *e22*] = -*e21*, [*e11*, *e13*] = -*e11*, [*e11*, *e18*] = -*e16*, [*e11*, *e23*] = -*e21*, [*e12*, *e13*] = -*e12*, [*e12*, *e18*] = -*e17*, [*e12*, *e23*] = -*e22*, [*e13*, *e14*] = *e14*, [*e13*, *e15*] = *e15*, [*e13*, *e18*] = -*e18*, [*e13*, *e23*] = -*e23*, [*e14*, *e16*] = *e11*, [*e14*, *e17*] = *e12*, [*e14*, *e18*] = *e13* - *e19*, [*e14*, *e19*] = *e14*, [*e14*, *e20*] = *e15*, [*e14*, *e23*] = -*e24*, [*e15*, *e18*] = -*e20*, [*e15*, *e21*] = *e11*, [*e15*, *e22*] = *e12*, [*e15*, *e23*] = *e13* - *e25*, [*e15*, *e24*] = *e14*, [*e15*, *e25*] = *e15*, [*e16*, *e19*] = -*e16*, [*e16*, *e24*] = -*e21*, [*e17*, *e19*] = -*e17*, [*e17*, *e24*] = -*e22*, [*e18*, *e19*] = -*e18*, [*e18*, *e24*] = -*e23*, [*e19*, *e20*] = *e20*, [*e19*, *e24*] = -*e24*, [*e20*, *e21*] = *e16*, [*e20*, *e22*] = *e17*, [*e20*, *e23*] = *e18*, [*e20*, *e24*] = *e19* - *e25*, [*e20*, *e25*] = *e20*, [*e21*, *e25*] = -*e21*, [*e22*,

```

    e25] = -e22, [e23, e25] = -e23, [e24, e25] = -e24]
> DGsetup(prL0) :
> # for j to 6 do print(LieBracket(e||j, add((a||i)·(e||i), i = 7..25))) :od
> S := -2 e7 - e8 + e19 + e25 :
    seq(LieBracket(S, e||i), i = 1..6)
                                -2 e1, -e2, -e3, 0 e1, e5, e6
(2)

> B := e16 - e22 :
    seq(LieBracket(B, e||i), i = 1..6)
                                0 e1, e5, -e6, 0 e1, 0 e1, 0 e1
(3)

> L1 := ChangeGradedComponent(pralg0, [ 0 = [S, B]], alg1)
L1 := [[e1, e7] = 2 e1, [e2, e3] = e1, [e2, e7] = e2, [e2, e8] = -e5, [e3, e7] = e3, [e3, e8] = e6,
[e5, e7] = -e5, [e6, e7] = -e6, [e7, e8] = 2 e8]
(4)

> DGsetup(L1) :
> LL := TanakaProlongation(alg1, 4, pralg1)
m:
    [[e1], [e2, e3, e4, e5, e6], [e7, e8]]
    [-2, -1, 0]
g^(1):
    [[e1], [e2, e3, e4, e5, e6], [e7, e8], [e9, e10]]
    [-2, -1, 0, 1]
LL := [[e1, e7] = 2 e1, [e1, e9] = -e5, [e1, e10] = -e6, [e2, e3] = e1, [e2, e7] = e2, [e2, e8] =
-e5, [e2, e10] = e8, [e3, e7] = e3, [e3, e8] = e6, [e3, e9] = e8, [e5, e7] = -e5, [e6, e7] =
-e6, [e7, e8] = 2 e8, [e7, e9] = 3 e9, [e7, e10] = 3 e10]
(5)

> DGsetup(LL) :
> seq(LieBracket(e9, e||i), i = 1..6); seq(LieBracket(e10, e||i), i = 1..6)
                                e5, 0 e1, -e8, 0 e1, 0 e1, 0 e1
                                e6, -e8, 0 e1, 0 e1, 0 e1, 0 e1
(6)

> LieAlgebraData([e7, e8, e9, e10])
                                [[e1, e2] = 2 e2, [e1, e3] = 3 e3, [e1, e4] = 3 e4]
(7)

```

Thus the prolongation is 10D with gradation dimensions (1[-2], 5[-1], 2[0], 1[1]).

To address/exclude the possibility of high symm dim we encode the possible structure equations of all filtered deformations of graded subalgebras up to dimension 7. Up to conjugation, we have the following 7 graded subalgebras (containing g[-]) of the maximal graded algebra:

(10D) R, X10, X01, Y, Z10, Z01, S, B, B10, B01;  
(9Ds) R, X10, X01, Y, Z10, Z01, S, B, k1\*B10+k2\*B01; (9Db) R, X10, X01, Y, Z10, Z01, B, B10, B01;  
(8Ds) R, X10, X01, Y, Z10, Z01, S, B; (8Db) R, X10, X01, Y, Z10, Z01, B, k1\*B10+k2\*B01;  
(7Ds) R, X10, X01, Y, Z10, Z01, S; (7Db) R, X10, X01, Y, Z10, Z01, B.

The following obtained knowledge is also encoded:

(i) Filtration: R (-2); X10, X01, Y, Z10, Z01 (-1); S, B (0); B10, B01 (+1) - this is not Freeman filtration but pullback contact filtration;  
(ii) brackets of vector fields from the structure relations (this involve Freeman filtration) can be used due to Lemma (this allows to change bracket of sections to bracket of symmetries with the minus sign like

passing from left-invariant vector fields to right-invariant vector fields; we remove the minus sign by passing to minus basis);

(iii) gradation of  $S$ , specified below, in the cases when  $S$  enters the graded subalgebra.

> # Notations :  $S = e_7 (= -\Lambda)$  has spectrum  $(-2, -1, -1, 0, 1, 1, 0, 2, 3, 3)$  in the basis  $(e_1, \dots, e_{10})$  and  $B = e_8, B_{10} = e_9, B_{01} = e_{10}$

Note that in all cases the stabilizer  $\mathfrak{g}_{\geq 0}$  is filtration deformation rigid, so we keep its brackets (either the action of  $S$ , when it is in, or the Abelian structure). Also, in the case, when  $S$  enters the graded subalgebra (it can be assumed to enter the filtered algebra with the same properties) the basis  $R, X_{10}, X_{01}, Y, Z_{10}, Z_{01}, S, B, B_{10}, B_{01}$  (or its subalgebra that contains  $\mathfrak{g}_{\geq 0}$  - transitivity) can be chosen almost uniquely because of the  $S$ -spectrum, except for  $Y$ , which is defined up to  $S$ . This makes  $S$  an (almost) grading element, and simplifies study of the cases of filtered deformations.

> # We use that the filtration is preserved and that  $S$  is almost semi-simple (i.e. on the entire algebra mod  $Y$ ),

which allows to fix a basis (by doing its filtered deformation and using the values of  $S$  spectrum) except for  $Y$  that is defined mod  $S$  :  
indeed we have the structure relations :

$$[S, R] = -2R, [S, X_{10}] = -X_{10}, [S, X_{01}] = -X_{01}, [S, Y] = t_7 S, [S, Z_{10}] = Z_{10}, [S, Z_{01}] = Z_{01}, [S, B] = 2B, [S, B_{10}] = 3B_{10}, [S, B_{01}] = 3B_{01},$$

(and if there are less  $B$  involved this line of relations is naturally reduced).

We want to indicate that the already obtained structure relations allow to fix  $S$  as grading (in Freeman filtration sense) element on the filtered algebra (note that if the stabilizer is reduced from 4D to lower-dimensional subalgebra, this computation still applied by equating to zero some of  $a[i]$ -coefficients)

> # `  $[Y, Z_{01}] = -Z_{10} + (c_1 + cc_1 + s_1) Z_{01} + a_1 S + a_2 B + a_3 B_{10} + a_4 B_{01}, [S, Y] = t S$   
 $\Rightarrow$   
 $[S, [Y, Z_{01}]] = [Y, Z_{01}] + t Z_{01}$   
 $= [S, -Z_{10} + (c_1 + cc_1 + s_1) Z_{01} + a_1 S + a_2 B + a_3 B_{10} + a_4 B_{01}]$   
 $= -Z_{10} + (c_1 + cc_1 + s_1) Z_{01} + 2a_2 B + 3a_3 B_{10} + 3a_4 B_{01} = -Z_{10} + (c_1 + cc_1 + s_1) Z_{01} + a_1 S + a_2 B + a_3 B_{10} + a_4 B_{01} + t Z_{01} \Rightarrow a[i] = t = 0$

or the same with LieAlgebras:

> restart : with (DifferentialGeometry) : with (LieAlgebras) : with (Tools) :  
Preferences ("ShowFramePrompt", false) :

> L := LieAlgebraData([ [Y, Z\_{10}] = (c\_1 + cc\_1 - s\_1) Z\_{10} - Z\_{01} + t\_1 S + t\_2 B + t\_3 B\_{10} + t\_4 Z\_{01},  
 $[Y, Z_{01}] = -Z_{10} + (c_1 + cc_1 + s_1) Z_{01} + t_1 S + t_2 B + t_4 B_{10} + t_5 Z_{01}, [Z_{10}, Z_{01}] = s_3 Z_{10} - ss_3 Z_{01} + t_5 B,$   
 $[S, Y] = t_0 S, [S, Z_{10}] = Z_{10}, [S, Z_{01}] = Z_{01}, [S, B] = 2B, [S, B_{10}] = 3B_{10}, [S, B_{01}] = 3B_{01},$   
 $[B, Y] = t_6 B + t_7 B_{10} + t_7 B_{01}, [B, Z_{10}] = t_8 B_{10} + t_9 B_{01}, [B, Z_{01}] = t_9 B_{10} + t_8 B_{01},$   
 $[B_{10}, Y] = t_{10} B_{10} + t_{11} B_{01}, [B_{01}, Y] = t_{11} B_{10} + t_{10} B_{01},$   
 $[Y, Z_{10}, Z_{01}, S, B, B_{10}, B_{01}], \text{alg}) :$

> DGsetup(L) :

> Jac := (X, Y, Z) → simplify(evalDG(LieBracket(X, LieBracket(Y, Z)) + LieBracket(Y, LieBracket(Z, X)) + LieBracket(Z, LieBracket(X, Y)))) :

> Jac(e1, e2, e4)

$$-t_0 e_2 - t_1 e_4 + t_2 e_5 + 2 t_3 e_6$$

(8)

This implies that all structure relations can be taken  $S$ -graded, and simplify commutation relations.

Note that we use the relations defining the basis uniquely except for  $Y$  that is defined mod  $S$ . Also,  $R =$

[X10,X01] is the defining relation of R.

We first consider those 4 cases, where S enters the subalgebra:

(10D)

```
> restart : with (DifferentialGeometry) : with (LieAlgebras) : with (Tools) :
Preferences ("ShowFramePrompt", 'false') :
> L := LieAlgebraData ([ [X10, X01] = I R,
[X10, Y] = (c1 - dd1) X10 - X01 + (c3 - dd3) Z10, [X01, Y] = -X10 + (cc1 - d1) X01
+ (cc3 - d3) Z01,
[X10, Z10] = -cc4 X10 - cc5 Z10 + t1 S, [X10, Z01] = -Y - dd6 X10 - dd7 Z10 - dd8 Z01
+ t2 S,
[X01, Z10] = -Y - d6 X01 - d8 Z10 - d7 Z01 + tt2 S, [X01, Z01] = -c4 X01 - c5 Z01
+ tt1 S,
[Y, Z10] = -(c6 + d10) Z10 - Z01, [Y, Z01] = -Z10 - (cc6 + dd10) Z01,
[Z10, Z01] = s3 Z10 - ss3 Z01 + t3 B,
[Y, R] = t4 R, [Z10, R] = t5 X10 + t6 X01, [Z01, R] = tt6 X10 + tt5 X01,
[S, R] = -2 R, [S, X10] = -X10, [S, X01] = -X01, [S, Z10] = Z10, [S, Z01] = Z01, [S, B]
= 2 B, [S, B10] = 3 B10, [S, B01] = 3 B01,
[B, R] = t8 Y + t9 S, [B, X10] = I Z10, [B, X01] = -I Z01, [B, Y] = t10 B, [B, Z10] = t11 B10
+ t12 B01, [B, Z01] = tt12 B10 + tt11 B01,
[B10, R] = Z10, [B10, X01] = -B, [B10, Y] = t14 B10 + t15 B01,
[B01, R] = Z01, [B01, X10] = -B, [B01, Y] = tt15 B10 + tt16 B01,
[R, X10, X01, Y, Z10, Z01, S, B, B10, B01], alg) :
```

```
> DGsetup(L) :
```

```
> JC := Query( {a}, "Jacobi") : JC[1] : JCC := JC[2] : nops(JCC)
false
```

191

(9)

```
> JCC[1..20]
```

```
{c4, c5, cc4, cc5, d6, d7, d8, dd6, dd7, dd8, s3, ss3, t15, tt15, -I c4, -I ss3, I cc4, I d6, I dd6,
I s3}
```

(10)

```
> s11 := solve(JCC[1..20]) : JCC1 := simplify(eval(JCC, s11)) :
```

```
> JCC1[1..10]
```

```
{-1, 0, 1, -I (t8 - 2), -I (t2 + t9 + tt2), -I (c1 - c6 - d10 - dd1 + t10), -I (c1 + cc1
- d1 - dd1 + t4), -I (-cc1 + cc6 + d1 + dd10 - t10), t6 (cc3 - d3), t8 (-cc3 + d3)}
```

(11)

```
>
```

(9Ds)

```
> restart : with (DifferentialGeometry) : with (LieAlgebras) : with (Tools) :
Preferences ("ShowFramePrompt", 'false') :
```

```
> L := LieAlgebraData ([ [X10, X01] = I R,
[X10, Y] = (c1 - dd1) X10 - X01 + (c3 - dd3) Z10, [X01, Y] = -X10 + (cc1 - d1) X01
+ (cc3 - d3) Z01,
[X10, Z10] = -cc4 X10 - cc5 Z10 + t1 S, [X10, Z01] = -Y - dd6 X10 - dd7 Z10 - dd8 Z01
+ t2 S,
[X01, Z10] = -Y - d6 X01 - d8 Z10 - d7 Z01 + tt2 S, [X01, Z01] = -c4 X01 - c5 Z01
+ tt1 S,
[Y, Z10] = -(c6 + d10) Z10 - Z01, [Y, Z01] = -Z10 - (cc6 + dd10) Z01,
```

$[Z10, Z01] = s3 Z10 - ss3 Z01 + t3 B,$   
 $[Y, R] = t4 R, [Z10, R] = t5 X10 + t6 X01, [Z01, R] = tt6 X10 + tt5 X01,$   
 $[S, R] = -2 R, [S, X10] = -X10, [S, X01] = -X01, [S, Z10] = Z10, [S, Z01] = Z01, [S, B]$   
 $= 2 B, [S, B1] = 3 B1,$   
 $[B, R] = t8 Y + t9 S, [B, X10] = I Z10, [B, X01] = -I Z01, [B, Y] = t10 B, [B, Z10] = t11 B1,$   
 $[B, Z01] = tt11 B1,$   
 $[B1, R] = r1 Z10 + r2 Z01, [B1, X10] = r3 B, [B1, X01] = r4 B, [B1, Y] = t12 B1,$   
 $[R, X10, X01, Y, Z10, Z01, S, B, B1], alg) :$

> DGsetup(L) :

> JC := Query({a}, "Jacobi") : JC[1] ; JCC := JC[2] : nops(JCC)

*false*

172

(12)

> JCC[1..13]

*{c5, cc5, d7, d8, dd7, dd8, s3, -I c4, -I ss3, I cc4, I d6, I dd6, I s3}*

(13)

> sl1 := solve(JCC[1..7]) : JCC1 := simplify(eval(JCC, sl1)) :

> JCC1[1..16]

*{0, -I c4, -I ss3, -I (d6 + ss3), -I (r1 + r4), -I (r2 + r3), -I (t8 - 2), -I (t2 + t9*  
 $+ tt2), -I (c1 - c6 - d10 - dd1 + t10), -I (c1 + cc1 - d1 - dd1 + t4), -I (-cc1$   
 $+ cc6 + d1 + dd10 - t10), I cc4, I d6, I dd6, I (c4 + dd6), I (cc4 + d6)}$

(14)

> sl2 := solve(JCC1[1..16]) : JCC2 := simplify(eval(JCC1, sl2)) :

> JCC2[1..36]

*{0, t6 (cc3 - d3), tt6 (c3 - dd3), (c3 - dd3) t3, (c3 - dd3) t5, (c3 - dd3) t6, (-cc3*

(15)

$+ d3) t3, (-cc3 + d3) tt11, (cc3 - d3) tt5, (cc3 - d3) tt6, -3 r3, -3 r4,$

$-\frac{t3 (cc6 + dd10 - t4 + c6 + d10)}{2}, -\frac{t9 (cc6 + dd10 - t4 + c6 + d10)}{2}, -(c3$

$- dd3) t11, -2 c3 + 2 dd3, c3 - dd3, -2 cc3 + 2 d3, -cc3 + d3, -2 t1 - I t6, t1 - 1,$

$-2 tt1 + I tt6, -tt1 + 1, -I t6 + 2, I tt6 + 2, (-t3 + tt5) r4 + tt6 r3, (t3 + t5) r3$

$+ t6 r4, (-2 t9 - tt2) r3 + r4 t1, (-t9 + tt2) r4 + r3 tt1, (c3 - d3 + cc3 - dd3) tt2$

$- t9 (-cc3 + d3), (-c6 - t4 - d10 + t12) r4 - r3, (c6 + t4 + d10 - t12) r4 + r3, ($

$-t4 - cc6 + t12 - dd10) r3 - r4, (t4 + cc6 - t12 + dd10) r3 + r4,$

$\frac{(c6 + t4 + 3 cc6 + d10 - 2 t12 + 3 dd10) tt11}{2} + tt11,$

$\frac{(3 c6 + t4 + cc6 + 3 d10 - 2 t12 + dd10) tt11}{2} + tt11 \}$

```

> sl3 := solve({-3 r3, -3 r4, -2 c3 + 2 dd3, c3 - dd3, -2 cc3 + 2 d3, -cc3 + d3, -2 t1
- I t6, t1 - 1, -2 tt1 + I tt6, -tt1 + 1}): JCC3 := simplify(eval(JCC2, sl3)):
> JCC3[1..7]
{ -2, 0, 2, 3, 4, -  $\frac{t3 (cc6 + dd10 - t4 + c6 + d10)}{2}$ , -  $\frac{t9 (cc6 + dd10 - t4 + c6 + d10)}{2}$  } (16)

```

(8Ds)

```

> restart : with (DifferentialGeometry) : with (LieAlgebras) : with (Tools) :
Preferences ("ShowFramePrompt", 'false') :
> L := LieAlgebraData([ [X10, X01] = I R,
[X10, Y] = (c1 - dd1) X10 - X01 + (c3 - dd3) Z10, [X01, Y] = -X10 + (cc1 - d1) X01
+ (cc3 - d3) Z01,
[X10, Z10] = -cc4 X10 - cc5 Z10 + t1 S, [X10, Z01] = -Y - dd6 X10 - dd7 Z10 - dd8 Z01
+ t2 S,
[X01, Z10] = -Y - d6 X01 - d8 Z10 - d7 Z01 + tt2 S, [X01, Z01] = -c4 X01 - c5 Z01
+ tt1 S,
[Y, Z10] = -(c6 + d10) Z10 - Z01, [Y, Z01] = -Z10 - (cc6 + dd10) Z01,
[Z10, Z01] = s3 Z10 - ss3 Z01 + t3 B,
[Y, R] = t4 R, [Z10, R] = t5 X10 + t6 X01, [Z01, R] = tt6 X10 + tt5 X01,
[S, R] = -2 R, [S, X10] = -X10, [S, X01] = -X01, [S, Z10] = Z10, [S, Z01] = Z01, [S, B]
= 2 B,
[B, R] = t8 Y + t9 S, [B, X10] = I Z10, [B, X01] = -I Z01, [B, Y] = t10 B,
[R, X10, X01, Y, Z10, Z01, S, B], alg) :
> DGsetup(L) :
> JC := Query({a}, "Jacobi") : JC[1]; JCC := JC[2] : nops(JCC)
false
132 (17)

```

```

> JCC[1..13]
{c5, cc5, d7, d8, dd7, dd8, s3, -I c4, -I ss3, I cc4, I d6, I dd6, I s3} (18)

```

```

> sl1 := solve(JCC[1..7]) : JCC1 := simplify(eval(JCC, sl1)) :
> JCC1[1..13]
{0, -I c4, -I ss3, -I (d6 + ss3), -I (t8 - 2), -I (t2 + t9 + tt2), -I (c1 + cc1 - d1 - dd1
+ t4), I cc4, I d6, I dd6, I (c4 + dd6), I (cc4 + d6), I (-c1 + c6 + d10 + dd1 - t10)} (19)

```

```

> sl2 := solve(JCC1[1..13]) : JCC2 := simplify(eval(JCC1, sl2)) :
> JCC2[1..31]
{0, I (cc1 - cc6 - d1 - dd10 + t10), t3 (t4 + cc1 - cc6 - dd10 - d1), t6 (cc3 - d3), tt6 (c3 - dd3), (c3 - dd3) t3, (c3 - dd3) t5, (c3 - dd3) t6, (cc3 - d3) tt5, (cc3 - d3) tt6, 2 t1,
2 tt1, -t9 (t10 - t4), -(cc3 - d3) t3, -2 - I t6, -2 + I tt6, -2 c3 + 2 dd3, c3 - dd3,
-2 cc3 + 2 d3, -cc3 + d3, -2 t1 - I t6, t1 - 1, -2 t10 + 2 t4, -t10 + t4, -2 tt1 + I tt6,
-tt1 + 1, -I t6 + 2, I tt6 + 2, (-d3 + cc3 - dd3 + c3) tt2 - t9 (-cc3 + d3), t1 - 1
- I t6, 2 t3 + t5 - tt5} (20)

```

```

> sl3 := solve({I (cc1 - cc6 - d1 - dd10 + t10), 2 t1, 2 tt1, -2 - I t6, -2 + I tt6, -2 c3
+ 2 dd3, c3 - dd3, -2 cc3 + 2 d3, -cc3 + d3}): JCC3 := simplify(eval(JCC2, sl3)) :

```

```
> JCC3[1..10]
{-1, 0, 1, 2, 4, t3 (-t10 + t4), (t10 - t4) t2, -t9 (t10 - t4), -(t10 - t4) t5, -(t10
- t4) t5}
```

(7Ds)

```
> restart : with (DifferentialGeometry) : with (LieAlgebras) : with (Tools) :
Preferences ("ShowFramePrompt", false) :
> L := LieAlgebraData ([ [X10, X01] = I R,
[X10, Y] = (c1 - dd1) X10 - X01 + (c3 - dd3) Z10, [X01, Y] = -X10 + (cc1 - d1) X01
+ (cc3 - d3) Z01,
[X10, Z10] = -cc4 X10 - cc5 Z10 + t1 S, [X10, Z01] = -Y - dd6 X10 - dd7 Z10 - dd8 Z01
+ t2 S,
[X01, Z10] = -Y - d6 X01 - d8 Z10 - d7 Z01 + t2 S, [X01, Z01] = -c4 X01 - c5 Z01
+ t1 S,
[Y, Z10] = -(c6 + d10) Z10 - Z01, [Y, Z01] = -Z10 - (cc6 + dd10) Z01,
[Z10, Z01] = s3 Z10 - ss3 Z01,
[Y, R] = t4 R, [Z10, R] = t5 X10 + t6 X01, [Z01, R] = t6 X10 + t5 X01,
[S, R] = -2 R, [S, X10] = -X10, [S, X01] = -X01, [S, Z10] = Z10, [S, Z01] = Z01 ],
[R, X10, X01, Y, Z10, Z01, S], alg) :
```

```
> DGsetup(L) :
```

```
> JC := Query({a}, "Jacobi") : JC[1] : JCC := JC[2] : nops(JCC)
```

false

97

(22)

```
> JCC[1..7]
```

{c5, cc5, d7, d8, dd7, dd8, s3}

(23)

```
> sl1 := solve(JCC[1..6]) : JCC1 := simplify(eval(JCC, sl1)) :
```

```
> JCC1[1..5]
```

{0, s3, -I (c1 + cc1 - d1 - dd1 + t4), I (c4 + dd6), I (cc4 + d6)}

(24)

```
> sl2 := solve(JCC1[1..5]) : JCC2 := simplify(eval(JCC1, sl2)) :
```

```
> JCC2[1..40]
```

```
{0, d6, dd6, dd6 (c3 - dd3), dd6 (-cc3 + d3), ss3 dd6, t6 (cc3 - d3), t6 (c3 - dd3), (-c3
+ dd3) d6, (c3 - dd3) t5, (c3 - dd3) t6, (c6 + d10) ss3, (cc3 - d3) dd6, (cc3 - d3) t5,
(cc3 - d3) t6, (ss3 + d6) (cc3 - d3), -2 d6, -d6, 2 d6, -2 dd6, -dd6, 2 dd6, -ss3,
-ss3 dd6, -ss3 (c3 - dd3), -2 c3 + 2 dd3, c3 - dd3, -2 cc3 + 2 d3, -cc3 + d3, -ss3
-d6, -2 t1 - I t6, t1 - 1, -2 t1 + I t6, -t1 + 1, -t5 + t5, (-c6 - d10) d6 + dd6,
(c6 + d10) d6 - dd6, -(cc3 - d3) t2 + (c3 - dd3) t2, (-cc6 - dd10) dd6 + d6, (cc6
+ dd10) dd6 - d6}
```

(25)

```
> sl3 := solve({0, d6, dd6, -ss3, -2 c3 + 2 dd3, c3 - dd3, -2 cc3 + 2 d3, -cc3 + d3, -ss3
-d6, -2 t1 - I t6, t1 - 1, -2 t1 + I t6, -t1 + 1, -t5 + t5}) : JCC3 :=
simplify(eval(JCC2, sl3)) :
```

```
> JCC3[1..6]
```

```
{-2, 0, 2, (c6 + d10 + cc1 - d1) t2, (cc1 - cc6 - dd10 - d1 + t4) t5, -(c6 + d10 + cc1
-d1) t5}
```

(26)

Now we concentrate on the remaining 3 cases, where the grading element  $S$  does not enter the subalgebra.

In this case the deformation is unrestricted, and we will have to add all higher filtrands terms to the brackets with new independent coefficients as parameters. This gives a large number of parameters, yet the Jacobi condition rules out all such possibilities.

(9Db)

```
> restart : with(DifferentialGeometry) : with(LieAlgebras) : with(Tools) :
Preferences("ShowFramePrompt",false) :
> L := LieAlgebraData([ [X10, X01] = I R,
[X10, Y] = (c1 - dd1) X10 - X01 + (c3 - dd3) Z10 + t1 B + t2 B10 + t3 B01,
[X01, Y] = -X10 + (cc1 - d1) X01 + (cc3 - d3) Z01 + tt1 B + tt3 B10 + tt2 B01,
[X10, Z10] = -cc4 X10 - cc5 Z10 + t4 B + t5 B10 + t6 B01,
[X10, Z01] = -Y - dd6 X10 - dd7 Z10 - dd8 Z01 + t7 B + t8 B10 + t9 B01,
[X01, Z10] = -Y - d6 X01 - d8 Z10 - d7 Z01 + tt7 B + tt9 B10 + tt8 B01,
[X01, Z01] = -c4 X01 - c5 Z01 + tt4 B + tt6 B10 + tt5 B01,
[Y, Z10] = -(c6 + d10) Z10 - Z01 + t10 B + t11 B10 + t12 B01,
[Y, Z01] = -Z10 - (cc6 + dd10) Z01 + tt10 B + tt12 B10 + tt11 B01,
[Z10, Z01] = s3 Z10 - ss3 Z01 + t13 B + t14 B10 - tt14 B01,
[X10, R] = r1 R + r2 X10 + r3 X01 + r4 Y + r5 Z10 + r6 Z01 + r7 B + r8 B10 + r9 B01,
[X01, R] = r10 R + r11 X10 + r12 X01 + r13 Y + r14 Z10 + r15 Z01 + r16 B + r17 B10
+ r18 B01,
[Y, R] = r19 R + r20 X10 + r21 X01 + r22 Y + r23 Z10 + r24 Z01 + r25 B + r26 B10
+ r27 B01,
[Z10, R] = r28 R + r29 X10 + r30 X01 + r31 Y + r32 Z10 + r33 Z01 + r34 B + r35 B10
+ r36 B01,
[Z01, R] = r37 R + r38 X10 + r39 X01 + r40 Y + r41 Z10 + r42 Z01 + r43 B + r44 B10
+ r45 B01,
[B, R] = r46 X10 + r47 X01 + r48 Y + r49 Z10 + r50 Z01 + r51 B + r52 B10 + r53 B01,
[B, X10] = I Z10 + t15 B + t16 B10 + t17 B01,
[B, X01] = -I Z01 - tt15 B - tt17 B10 - tt16 B01,
[B, Y] = t17 B + t18 B10 - tt18 B01,
[B, Z10] = r54 B + t19 B10 + t20 B01, [B, Z01] = r55 B + tt20 B10 + tt19 B01,
[B10, R] = Z10 + t21 B + t22 B10 + t23 B01,
[B10, X10] = t24 B10 + t25 B01, [B10, X01] = -B + t26 B10 + t27 B01, [B10, Y] = t28 B10
+ t29 B01,
[B10, Z10] = t30 B10 + t31 B01, [B10, Z01] = t32 B10 + t33 B01,
[B01, R] = Z01 + tt21 B + tt23 B10 + tt22 B01,
[B01, X10] = -B + tt27 B10 + tt26 B01, [B01, X01] = tt25 B10 + tt24 B01, [B01, Y] = tt29 B10
+ tt28 B01,
[B01, Z10] = tt33 B10 + tt32 B01, [B01, Z01] = tt31 B10 + tt32 B01 ],
[R, X10, X01, Y, Z10, Z01, B, B10, B01], alg) :
```

```
> DGsetup(L) :
```

```
> JC := Query({a}, "Jacobi") : JC[1] ; JCC := JC[2] : nops(JCC)
```

false

378

(27)

```
> JCC[1..20]
```

```
{c4, cc4, r46, r47, t31, t33, tt31, tt33, -I ss3, -I t32, -I t33, -I tt31, -I tt32, I s3, I t30, I t31, (28)
```



$I\ t32, I\ t33, -t25, -t31\}$

```
> s11 := solve(JCC[1..20]) : JCC1 := simplify(eval(JCC, s11)) :
> JCC1[1..30]
{-1, 0, 1, d6, dd6, r28, r37, t29, -I r28, -I r54, -I (d6 - r54), -I (r12 + r2), -I (r48
- 2), -I (c1 - c6 - d10 - dd1 + t17), -I (c1 + cc1 - d1 - dd1 + r19), -I (d1 + cc6
- cc1 - t17 + dd10), I d6, I dd6, I r37, I r55, I (d6 - r28), I (dd6 - r37), I (dd6 - r55),
I (d7 + dd8 - r50 - t15), I (d8 + dd7 - r49 + t15), r48 (r19 - t17), r48 (-r54
+ r28), r48 (-r55 + r37), -d6, -dd6}
```

(8Db)

```
> restart : with (DifferentialGeometry) : with (LieAlgebras) : with (Tools) :
Preferences ("ShowFramePrompt", false) :
> L := LieAlgebraData ([ [X10, X01] = I R,
[X10, Y] = (c1 - dd1) X10 - X01 + (c3 - dd3) Z10 + t1 B + t2 B1,
[X01, Y] = -X10 + (cc1 - d1) X01 + (cc3 - d3) Z01 + tt1 B + t3 B1,
[X10, Z10] = -cc4 X10 - cc5 Z10 + t4 B + t6 B1,
[X10, Z01] = -Y - dd6 X10 - dd7 Z10 - dd8 Z01 + t5 B + t7 B1,
[X01, Z10] = -Y - d6 X01 - d8 Z10 - d7 Z01 + tt5 B + t8 B1,
[X01, Z01] = -c4 X01 - c5 Z01 + tt4 B + t9 B1,
[Y, Z10] = -(c6 + d10) Z10 - Z01 + t10 B + t11 B1,
[Y, Z01] = -Z10 - (cc6 + dd10) Z01 + tt10 B + t12 B1,
[Z10, Z01] = s3 Z10 - ss3 Z01 + t13 B + t14 B1,
[X10, R] = r1 R + r2 X10 + r3 X01 + r4 Y + r5 Z10 + r6 Z01 + r7 B + r8 B1,
[X01, R] = r9 R + r10 X10 + r11 X01 + r12 Y + r13 Z10 + r14 Z01 + r15 B + r16 B1,
[Y, R] = r17 R + r18 X10 + r19 X01 + r20 Y + r21 Z10 + r22 Z01 + r23 B + r24 B1,
[Z10, R] = r25 R + r26 X10 + r27 X01 + r28 Y + r29 Z10 + r30 Z01 + r31 B + r32 B1,
[Z01, R] = r33 R + r34 X10 + r35 X01 + r36 Y + r37 Z10 + r38 Z01 + r39 B + r40 B1,
[B, R] = r41 X10 + r42 X01 + r43 Y + r44 Z10 + r45 Z01 + r46 B + r47 B1,
[B, X10] = I Z10 + t15 B + t16 B1,
[B, X01] = -I Z01 - tt15 B + t17 B1,
[B, Y] = t18 B + t19 B1,
[B, Z10] = t20 B + t21 B1, [B, Z01] = tt20 B + t22 B1,
[B1, R] = k1 Z10 + k2 Z01 + t23 B + t24 B1,
[B1, X10] = -k2 B + t25 B1, [B10, X01] = -k1 B + t26 B1, [B10, Y] = t27 B1,
[B1, Z10] = t28 B1, [B1, Z01] = t29 B1,
[R, X10, X01, Y, Z10, Z01, B, B1], alg) :
> DGsetup(L) :
> JC := Query({a}, "Jacobi") : JC[1]; JCC := JC[2] : nops(JCC)
false
263
(30)
> JCC[1..26]
{-I ss3, -I t29, I s3, I t28, k1 r41, k2 r42, 2 I - I r43, -c4 + dd6, c4 - dd6, -d6 + cc4, d6
- cc4, s3 - c4, -ss3 + cc4, -I r11 - I r2, -I r25 - I r42, -I t20 + I cc4, I d6 - I r42,
I dd6 - I r41, I r33 + I r41, I tt20 - I c4, t16 k1 - I t24, -c5 + dd7 - I r36, c5 - d8
+ dd7, -d7 + cc5 - I r28, -dd8 + cc5 + d7, -I r18 + dd6 cc3 - dd6 d3}
```

(31)

```

> sll := solve(JCC[1..26]) : JCC1 := simplify(eval(JCC, sll)) :
> JCC1[1..10]
{-1, 0, 1, -I r19, -I r27, -I (c1 + cc1 - d1 - dd1 + r17), I r34, I (-c1 + c6 + d10 + dd1 (32)
- t18), I (cc1 - cc6 - d1 - dd10 + t18), k1 (d8 + r44 + r9 - t26)}

```

(7Db)

```

> restart : with (DifferentialGeometry) : with (LieAlgebras) : with (Tools) :
Preferences ("ShowFramePrompt", false) :
> L := LieAlgebraData ([ [X10, X01] = I R,
[X10, Y] = (c1 - dd1) X10 - X01 + (c3 - dd3) Z10 + t1 B,
[X01, Y] = -X10 + (cc1 - d1) X01 + (cc3 - d3) Z01 + tt1 B,
[X10, Z10] = -cc4 X10 - cc5 Z10 + t4 B,
[X10, Z01] = -Y - dd6 X10 - dd7 Z10 - dd8 Z01 + t5 B,
[X01, Z10] = -Y - d6 X01 - d8 Z10 - d7 Z01 + tt5 B,
[X01, Z01] = -c4 X01 - c5 Z01 + tt4 B,
[Y, Z10] = -(c6 + d10) Z10 - Z01 + t10 B,
[Y, Z01] = -Z10 - (cc6 + dd10) Z01 + tt10 B,
[Z10, Z01] = s3 Z10 - ss3 Z01 + t13 B,
[X10, R] = r1 R + r2 X10 + r3 X01 + r4 Y + r5 Z10 + r6 Z01 + r7 B,
[X01, R] = r8 R + r9 X10 + r10 X01 + r11 Y + r12 Z10 + r13 Z01 + r14 B,
[Y, R] = r15 R + r16 X10 + r17 X01 + r18 Y + r19 Z10 + r20 Z01 + r21 B,
[Z10, R] = r22 R + r23 X10 + r24 X01 + r25 Y + r26 Z10 + r27 Z01 + r28 B,
[Z01, R] = r29 R + r30 X10 + r31 X01 + r32 Y + r33 Z10 + r34 Z01 + r35 B,
[B, R] = r36 X10 + r37 X01 + r38 Y + r39 Z10 + r40 Z01 + r41 B,
[B, X10] = I Z10 + t6 B,
[B, X01] = -I Z01 - tt6 B,
[B, Y] = t7 B,
[B, Z10] = t8 B, [B, Z01] = tt8 B,
[R, X10, X01, Y, Z10, Z01, B], alg) :
> DGsetup(L) :
> JC := Query({a}, "Jacobi") : JC[1]; JCC := JC[2] : nops(JCC)
false
181 (33)

```

```

> JCC[1..20]
{-I ss3, I s3, 2 I - I r38, -c4 + dd6, c4 - dd6, -d6 + cc4, d6 - cc4, s3 - c4, -ss3 + cc4, (34)
-I r10 - I r2, -I r22 - I r37, -I t8 + I cc4, I d6 - I r37, I dd6 - I r36, I r29 + I r36, I tt8
-I c4, -c5 + dd7 - I r32, c5 - d8 + dd7, -d7 + cc5 - I r25, -dd8 + cc5 + d7}

```

```

> sll := solve(JCC[1..20]) : JCC1 := simplify(eval(JCC, sll)) :
> JCC1[1..10]
{-1, 0, 1, -I r16, -I r17, -I r24, -I (r41 + t5 + tt5), -I (c1 - c6 - d10 - dd1 + t7), (35)
-I (c1 + cc1 - d1 - dd1 + r15), I r30}

```

Conclusion: in all cases of filtered deformation of the 6D orbit on 3ndg 7D CR of type  $\dim(U\_L)=2$ ,  $\dim(U\_K)=3$ , the ideal of Jacobi identity relations contains element 1, hence the algebra is not realizable.

>

Now we compute the Tanaka prolongation of the 6D orbit on 3ndg 7D CR of type  $\dim(U\_L)=1$ ,  $\dim$

(U\_K)=3, with 2D structure reduction

```
> restart : with (DifferentialGeometry) : with (LieAlgebras) : with (GroupActions) : with (Tools) :
Preferences ("ShowFramePrompt", false) :
```

```
> L := LieAlgebraData ([ [X10, X01] = R], [R, X10, X01, Y10, Y01, Z], alg, grading = [-2, -1,
-1, -1, -1, -1]) :
```

```
> DGsetup(L) :
```

```
> infolevel[TanakaProlongation] := 2 :
```

```
> prL0 := TanakaProlongation(alg, 1, pralg0)
```

```
m:
```

```
[[e1], [e2, e3, e4, e5, e6]]
[-2, -1]
```

```
g^(0):
```

```
[[e1], [e2, e3, e4, e5, e6], [e7, e8, e9, e10, e11, e12, e13,
e14, e15, e16, e17, e18, e19, e20, e21, e22, e23, e24, e25]]
[-2, -1, 0]
```

```
prL0 := [[e1, e7] = -e1, [e2, e3] = e1, [e2, e8] = -e2, [e2, e10] = -e3, [e2, e11] = -e4,
[e2, e16] = -e5, [e2, e21] = -e6, [e3, e7] = -e3, [e3, e8] = e3, [e3, e9] = -e2, [e3, e12]
= -e4, [e3, e17] = -e5, [e3, e22] = -e6, [e4, e13] = -e4, [e4, e18] = -e5, [e4, e23] =
-e6, [e5, e14] = -e4, [e5, e19] = -e5, [e5, e24] = -e6, [e6, e15] = -e4, [e6, e20] =
-e5, [e6, e25] = -e6, [e7, e9] = -e9, [e7, e10] = e10, [e7, e12] = -e12, [e7, e17] =
-e17, [e7, e22] = -e22, [e8, e9] = 2 e9, [e8, e10] = -2 e10, [e8, e11] = -e11, [e8, e12]
= e12, [e8, e16] = -e16, [e8, e17] = e17, [e8, e21] = -e21, [e8, e22] = e22, [e9, e10]
= e8, [e9, e11] = -e12, [e9, e16] = -e17, [e9, e21] = -e22, [e10, e12] = -e11, [e10,
e17] = -e16, [e10, e22] = -e21, [e11, e13] = -e11, [e11, e18] = -e16, [e11, e23] =
-e21, [e12, e13] = -e12, [e12, e18] = -e17, [e12, e23] = -e22, [e13, e14] = e14, [e13,
e15] = e15, [e13, e18] = -e18, [e13, e23] = -e23, [e14, e16] = e11, [e14, e17] = e12,
[e14, e18] = e13 - e19, [e14, e19] = e14, [e14, e20] = e15, [e14, e23] = -e24, [e15, e18]
= -e20, [e15, e21] = e11, [e15, e22] = e12, [e15, e23] = e13 - e25, [e15, e24] = e14,
[e15, e25] = e15, [e16, e19] = -e16, [e16, e24] = -e21, [e17, e19] = -e17, [e17, e24] =
-e22, [e18, e19] = -e18, [e18, e24] = -e23, [e19, e20] = e20, [e19, e24] = -e24, [e20,
e21] = e16, [e20, e22] = e17, [e20, e23] = e18, [e20, e24] = e19 - e25, [e20, e25] = e20,
[e21, e25] = -e21, [e22, e25] = -e22, [e23, e25] = -e23, [e24, e25] = -e24]
```

(36)

```
> DGsetup(prL0) :
```

```
> # for j to 6 do print(LieBracket(e||j, add((a||i)·(e||i), i = 7..25))) :od
```

```
> B := add(a||i·e||i, i in {seq(i, i = 7..12), 16, 17, 21, 22})
```

```
B := a7 e7 + a8 e8 + a9 e9 + a10 e10 + a11 e11 + a12 e12 + a16 e16 + a17 e17 + a21 e21
+ a22 e22 (37)
```

```
> DGinfo(LieBracket(B, e4), "CoefficientSet") union DGinfo(LieBracket(B, e5),
"CoefficientSet") union DGinfo(LieBracket(B, e6), "CoefficientSet")
{a13, a14, a15, a18, a19, a20, a23, a24, a25} (38)
```

```
> LieBracket(B, e2), LieBracket(B, e3)
```

(39)

$$a8 e2 + a10 e3 + a11 e4 + a16 e5 + a21 e6, a9 e2 + (-a8 + a7) e3 + a12 e4 + a17 e5 + a22 e6 \quad (39)$$

$$\begin{aligned} &> B := \exp\left(\frac{It}{2}\right) e11 + \exp\left(-\frac{It}{2}\right) e17 : \\ &> LieBracket(B, e4), LieBracket(B, e5), LieBracket(B, e6) \\ &\quad 0 e1, 0 e1, 0 e1 \end{aligned} \quad (40)$$

$$\begin{aligned} &> LieBracket(B, e2), LieBracket(B, e3) \\ &\quad e^{\frac{1}{2}t} e4, e^{-\frac{1}{2}t} e5 \end{aligned} \quad (41)$$

$$\begin{aligned} &> L1 := ChangeGradedComponent(pralg0, [0 = [B]], alg1) \\ &\quad L1 := \left[ [e2, e3] = e1, [e2, e7] = -e^{\frac{1}{2}t} e4, [e3, e7] = -e^{-\frac{1}{2}t} e5 \right] \end{aligned} \quad (42)$$

$$\begin{aligned} &> DGsetup(L1) : \\ &> LL := TanakaProlongation(alg1, 4, pralg1) \\ m: &\quad [[e1], [e2, e3, e4, e5, e6], [e7]] \\ &\quad [-2, -1, 0] \\ g^{(1)}: &\quad [[e1], [e2, e3, e4, e5, e6], [e7], [e8, e9]] \\ &\quad [-2, -1, 0, 1] \\ LL := &\quad \left[ [e1, e8] = -e4, [e1, e9] = -e5, [e2, e3] = e1, [e2, e7] = -e^{\frac{1}{2}t} e4, [e2, e9] = \right. \\ &\quad \left. -\frac{e7}{e^{-\frac{1}{2}t}}, [e3, e7] = -e^{-\frac{1}{2}t} e5, [e3, e8] = \frac{e7}{e^{\frac{1}{2}t}} \right] \end{aligned} \quad (43)$$

$$\begin{aligned} &> DGsetup(LL) : \\ &> seq(LieBracket(e8, e||i), i = 1..6); seq(LieBracket(e9, e||i), i = 1..6) \\ &\quad e4, 0 e1, -e^{-\frac{1}{2}t} e7, 0 e1, 0 e1, 0 e1 \\ &\quad e5, e^{\frac{1}{2}t} e7, 0 e1, 0 e1, 0 e1, 0 e1 \end{aligned} \quad (44)$$

$$\begin{aligned} &> LieAlgebraData([e7, e8, e9]) \\ &\quad [ ] \end{aligned} \quad (45)$$

>

Thus the prolonged graded algebra is 6+3=9 dimensional, and there are 3 graded subalgebras with full g [-]: those containing entire stabilizer [B,B10,B01], those containing [B,k1\*B10+k2\*B01] and only [B]. We consider these 3 cases in turn. The deformation is unrestricted (but we added the condition for integrability of the orbit distribution [R,X10,X01,Y10,Y01,Z] namely d8=c5+d7, d11=cc7), and we will have to add all higher filtrands terms to the brackets with new independent coefficients as parameters. This gives a large number of parameters, yet the Jacobi condition rules out all such possibilities.

(9D)

> restart : with (DifferentialGeometry) : with (LieAlgebras) : with (Tools) :  
 Preferences ("ShowFramePrompt", 'false') :

> L := LieAlgebraData ( [ [X10, X01] = R,  
 [X10, Y10] = c1 X10 + c2 Y10 + t1 B + t2 B10 + t3 B01,  
 [X10, Y01] = -dd1 X10 - X01 - dd2 Y10 - dd3 Y01 - dd4 Z + t4 B + t5 B10 + t6 B01,  
 [X01, Y10] = -X10 - d1 X01 - d3 Y10 - d2 Y01 - d4 Z + t4 B + t6 B10 + t5 B01,  
 [X01, Y01] = cc1 X01 + cc2 Y01 + t1 B + t3 B10 + t2 B01,  
 [X10, Z] = -(cc3 + dd5) X10 - (cc4 + dd6) Y10 - Y01 - dd8 Z + t7 B + t8 B10 + t9 B01,  
 [X01, Z] = -(c3 + d5) X01 - Y10 - (c4 + d6) Y01 - d8 Z + t7 B + t9 B10 + t8 B01,  
 [Y10, Y01] = exp(I t) Y10 - exp(-I t) Y01 + t10 B + t11 B10 + t12 B01,  
 [Y10, Z] = -(c6 + dd9) Y10 - c7 Z + t13 B + t14 B10 + t15 B01,  
 [Y01, Z] = -(cc6 + d9) Y01 - cc7 Z + t13 B + t15 B10 + t14 B01,  
 [X10, R] = r1 R + r2 X10 + r3 X01 + r4 Y10 + r5 Y01 + r6 Z + r7 B + r8 B10 + r9 B01,  
 [X01, R] = r10 R + r11 X10 + r12 X01 + r13 Y10 + r14 Y01 + r15 Z + r16 B + r17 B10  
 + r18 B01,  
 [Y10, R] = r19 R + r20 X10 + r21 X01 + r22 Y10 + r23 Y01 + r24 Z + r25 B + r26 B10  
 + r27 B01,  
 [Y01, R] = r28 R + r29 X10 + r30 X01 + r31 Y10 + r32 Y01 + r33 Z + r34 B + r35 B10  
 + r36 B01,  
 [Z, R] = r37 R + r38 X10 + r39 X01 + r40 Y10 + r41 Y01 + r42 Z + r43 B + r44 B10  
 + r45 B01,  
 [B, R] = r46 X10 + r47 X01 + r48 Y10 + r49 Y01 + r50 Z + r51 B + r52 B10 + r53 B01,  
 [B, X10] = exp ( ( I t / 2 ) ) Y10 + t16 B + t17 B10 + t18 B01,

$$\begin{aligned}
[B, X01] &= \exp\left(-\frac{It}{2}\right) Y01 + \pi16 B + \pi18 B10 + \pi17 B01, \\
[B, Y10] &= t19 B + t20 B10 + t21 B01, [B, Y01] = \pi19 B + \pi21 B10 + \pi20 B01, \\
[B, Z] &= t22 B + t23 B10 + t24 B01, \\
[B10, R] &= Y10 + t25 B + t26 B10 + t27 B01, \\
[B10, X10] &= t28 B10 + t29 B01, [B10, X01] = -\exp\left(-\frac{It}{2}\right) B + t30 B10 + t31 B01, \\
[B10, Y10] &= t32 B10 + t33 B01, [B10, Y01] = t34 B10 + t35 B01, [B10, Z] = t36 B10 \\
&+ t37 B01, \\
[B01, R] &= Y01 + \pi25 B + \pi27 B10 + \pi26 B01, \\
[B01, X10] &= \exp\left(\frac{It}{2}\right) B + \pi31 B10 + \pi30 B01, [B01, X01] = \pi29 B10 + \pi28 B01, \\
[B01, Y10] &= \pi35 B10 + \pi34 B01, [B01, Y01] = \pi33 B10 + \pi32 B01, [B01, Z] = \pi37 B10 \\
&+ \pi36 B01 \Big], \\
[R, X10, X01, Y10, Y01, Z, B, B10, B01], alg \Big):
\end{aligned}$$

$$\begin{aligned}
&> DGsetup(L) : \\
&> JC := Query(\{a\}, "Jacobi") : JC[1]; JCC := JC[2] : nops(JCC) \\
&\hspace{15em} false \\
&\hspace{15em} 383
\end{aligned} \tag{46}$$

$$\begin{aligned}
&> JCC[1..30] \\
&\left\{ t33 e^{\frac{1}{2}t}, t34 e^{-\frac{1}{2}t}, \pi33 e^{-\frac{1}{2}t}, \pi34 e^{\frac{1}{2}t}, \pi37 e^{-\frac{1}{2}t}, e^{-\frac{1}{2}t} t35, e^{-\frac{1}{2}t} \pi32, e^{-\frac{1}{2}t} (cc1 + t34 \right. \\
&\quad - \pi19), e^{-\frac{1}{2}t} (c3 - cc6 + d5 - d9 - t22), e^{\frac{1}{2}t} t32, e^{\frac{1}{2}t} \pi35, e^{\frac{1}{2}t} (dd1 + \pi19 - \pi32), \\
&\quad e^{\frac{1}{2}t} (cc3 + dd5 + t22 - \pi36), -c1, -c7, -cc1, -cc7, -t29, -t33, -t37, -\pi29, -\pi33, \\
&\quad -\pi37, -t33 e^{\frac{1}{2}t}, -t37 e^{\frac{1}{2}t}, -e^{-\frac{1}{2}t} cc7, -e^{-\frac{1}{2}t} (cc1 + \pi19), -e^{-\frac{1}{2}t} (d1 + t19 \\
&\quad \left. - t32), -e^{-\frac{1}{2}t} (c3 + d5 + t22 - \pi36), -e^{\frac{1}{2}t} c7 \right\}
\end{aligned} \tag{47}$$

$$\begin{aligned}
&> sll := solve(JCC[1..30]) : JCC1 := simplify(eval(JCC, sll)) : \\
&> JCC1[1..30] \\
&\left\{ -1, 0, r19, r28, t31, \pi31, r19 r47, r28 r46, r28 (2 t22 - t36), r46 (r37 - \pi36), r47 (r37 \right.
\end{aligned} \tag{48}$$

$$\begin{aligned} & -t36), t19 (c6 + dd9), t19 e^{\frac{1}{2}t}, t21 e^{\frac{1}{2}t}, tt21 e^{-\frac{1}{2}t}, (-3 t22 + 2 t36) tt21, (-2 t22 \\ & + t36) e^{1t}, (-3 t22 + t36 + tt36) tt20, e^{\frac{1}{2}t} r46, e^{\frac{1}{2}t} t20, e^{\frac{1}{2}t} tt21, -r28, -r19 (c6 \\ & + dd9), -t19 e^{\frac{1}{2}t}, -tt21 (cc2 + t30 - tt16), -tt21 e^{-\frac{1}{2}t}, -e^{-1t} (c6 + dd9), -e^{1t} t19, \\ & -e^{-\frac{1}{2}t} tt20, -e^{\frac{1}{2}t} r46 \} \end{aligned}$$

(8D) here B1=k1\*B10+k2\*B01 with k1,k2 not simultaneously zero

> restart : with (DifferentialGeometry) : with (LieAlgebras) : with (Tools) :  
Preferences ("ShowFramePrompt",false) :

> L := LieAlgebraData  $\left( \left[ \begin{aligned} & [X10, X01] = R, \\ & [X10, Y10] = c1 X10 + c2 Y10 + t1 B + t2 B1, \\ & [X10, Y01] = -dd1 X10 - X01 - dd2 Y10 - dd3 Y01 - dd4 Z + t4 B + t5 B1, \\ & [X01, Y10] = -X10 - d1 X01 - d2 Y01 - d3 Y10 - d4 Z + tt4 B + tt5 B1, \\ & [X01, Y01] = cc1 X01 + cc2 Y01 + tt1 B + tt2 B1, \\ & [X10, Z] = -(cc3 + dd5)X10 - (cc4 + dd6) Y10 - Y01 - dd8 Z + t7 B + t8 B1, \\ & [X01, Z] = -(c3 + d5) X01 - Y10 - (c4 + d6) Y01 - d8 Z + tt7 B + tt8 B1, \\ & [Y10, Y01] = \exp(I t) Y10 - \exp(-I t) Y01 + t10 B + t11 B1, \\ & [Y10, Z] = -(c6 + dd9) Y10 - c7 Z + t13 B + t14 B1, \\ & [Y01, Z] = -(cc6 + d9) Y01 - cc7 Z + tt13 B + tt14 B1, \\ & [X10, R] = r1 R + r2 X10 + r3 X01 + r4 Y10 + r5 Y01 + r6 Z + r7 B + r8 B1, \\ & [X01, R] = r10 R + r11 X10 + r12 X01 + r13 Y10 + r14 Y01 + r15 Z + r16 B + r17 B1, \\ & [Y10, R] = r19 R + r20 X10 + r21 X01 + r22 Y10 + r23 Y01 + r24 Z + r25 B + r26 B1, \\ & [Y01, R] = r28 R + r29 X10 + r30 X01 + r31 Y10 + r32 Y01 + r33 Z + r34 B + r35 B1, \\ & [Z, R] = r37 R + r38 X10 + r39 X01 + r40 Y10 + r41 Y01 + r42 Z + r43 B + r44 B1, \\ & [B, R] = r46 X10 + r47 X01 + r48 Y10 + r49 Y01 + r50 Z + r51 B + r52 B1, \end{aligned} \right. \right)$

$$[B, X10] = \exp\left(\frac{It}{2}\right) Y10 + t16 B + t17 Bl,$$

$$[B, X01] = \exp\left(-\frac{It}{2}\right) Y01 + t16 B + t17 Bl,$$

$$[B, Y10] = t19 B + t20 Bl, [B, Y01] = t19 B + t21 Bl,$$

$$[B, Z] = t22 B + t23 Bl,$$

$$[Bl, R] = k1 Y10 + k2 Y01 + t25 B + t26 Bl,$$

$$[Bl, X10] = k2 \exp\left(\frac{It}{2}\right) B + t28 Bl, [Bl, X01] = -k1 \exp\left(-\frac{It}{2}\right) B + t30 Bl,$$

$$[Bl, Y10] = t32 Bl, [Bl, Y01] = t34 Bl, [Bl, Z] = t36 Bl,$$

$$[R, X10, X01, Y10, Y01, Z, B, Bl], alg \Big):$$

> DGsetup(L) :

> JC := Query({a}, "Jacobi") : JC[1]; JCC := JC[2] : nops(JCC)  
false  
267

(49)

> JCC[1..30]

$$\left\{ k1 \left( e^{-\frac{1}{2}t} r50 + d4 \right), k1 (e^{1t} + r28 - t34), k1 \left( e^{-\frac{1}{2}t} r48 + d3 + r10 - t30 \right), k2 (e^{-1t} \right. \\ + r19 - t32), e^{-\frac{1}{2}t} t34, e^{-\frac{1}{2}t} (c3 - cc6 + d5 - d9 - t22), e^{\frac{1}{2}t} t32, k1 e^{-\frac{1}{2}t} (cc1 + t34 \\ - t19), k2 e^{\frac{1}{2}t} (cc3 + dd5 + t22 - t36), -k2 \left( e^{\frac{1}{2}t} r50 - dd4 \right), -k2 \left( e^{\frac{1}{2}t} r49 - dd3 \\ - r1 + t28 \right), -e^{-\frac{1}{2}t} cc7, -e^{-\frac{1}{2}t} (cc1 + t19), -e^{\frac{1}{2}t} c7, -e^{\frac{1}{2}t} (c1 + t19), -e^{\frac{1}{2}t} (c6 \\ - cc3 - dd5 + dd9 + t22), -k1 e^{-\frac{1}{2}t} (c3 + d5 + t22 - t36), -k2 e^{\frac{1}{2}t} (c1 - t19 \\ + t32), -r12 - r2, e^{-1t} cc7 - e^{1t} c7, -e^{-1t} r28 + e^{1t} r19, e^{-1t} t34 - e^{1t} t32, e^{-1t} t19 \\ - e^{1t} t19, -e^{-\frac{1}{2}t} r28 + r46, -e^{\frac{1}{2}t} r19 - r47, k1 e^{-\frac{1}{2}t} r46 + k1, -k2 e^{\frac{1}{2}t} r47 + k2, \\ \left. -c7 + e^{-1t} - c1, -cc1 + dd1 - r28, -cc7 + e^{1t} - cc1 \right\}$$

(50)

$$\begin{aligned} > sll := solve\left(\left\{ e^{-\frac{1}{2}t} t34, e^{-\frac{1}{2}t} (c3 - cc6 + d5 - d9 - t22), e^{\frac{1}{2}t} t32, -e^{-\frac{1}{2}t} cc7, \right. \right. \\ & \quad \left. -e^{-\frac{1}{2}t} (cc1 + t19), -e^{\frac{1}{2}t} c7, -e^{\frac{1}{2}t} (c1 + t19), -e^{\frac{1}{2}t} (c6 - cc3 - dd5 + dd9 + t22), \right. \\ & \quad \left. -r12 - r2, e^{-1t} cc7 - e^{1t} c7, -e^{-1t} r28 + e^{1t} r19, e^{-1t} t34 - e^{1t} t32, e^{-1t} t19 - e^{1t} t19, \right. \end{aligned}$$



$$\left. \begin{aligned} & -e^{-\frac{1}{2}t} r28 + r46, -e^{\frac{1}{2}t} r19 - r47, -c7 + e^{-1t} - c1, -cc1 + dd1 - r28, -cc7 + e^{1t} \\ & - cc1 \end{aligned} \right\} : JCC1 := \text{simplify}(\text{eval}(JCC, sl1)) :$$

> JCC1[1..30]

$$\begin{aligned} & \left\{ 0, kl \left( e^{21t} r19 + e^{1t} \right), kl \left( e^{-\frac{1}{2}t} r50 + d4 \right), kl \left( e^{-\frac{1}{2}t} r48 + d3 + r10 - t30 \right), k2 \left( e^{-1t} \right. \right. \\ & \quad \left. \left. + r19 \right), r19 \left( e^{\frac{31}{2}t} r19 + 3 e^{\frac{1}{2}t} \right), (cc6 + d9) e^{1t}, \left( -e^{\frac{1}{2}t} r50 + dd4 \right) k2, \left( -e^{-\frac{1}{2}t} \right. \right. \\ & \quad \left. \left. + (d1 - r19) e^{\frac{1}{2}t} \right) r19, \left( -e^{\frac{1}{2}t} r49 + dd3 + r1 - t28 \right) k2, e^{-1t} (cc3 + dd5 - t22), \right. \\ & \quad k2 e^{\frac{1}{2}t} (cc3 + dd5 + t22 - t36), e^{\frac{1}{2}t} r19 (cc6 + d9 - r37 + 2 t22), -d1 (cc3 + dd5 \\ & \quad - t22), -kl (cc3 + dd5 - r37 - t22 + t36), 2 kl e^{\frac{1}{2}t}, -k2 (cc6 + d9 - r37 + t36), \\ & \quad -2 k2 e^{-\frac{1}{2}t}, -r19 \left( e^{\frac{51}{2}t} r19 + 3 e^{\frac{31}{2}t} \right), -r19 (cc3 + dd5 - t22), -t20 (c2 - t16 \\ & \quad + t28), -t21 (cc2 + t30 - t16), -(cc6 + d9) e^{1t}, -(e^{21t} r19 + e^{1t}) (cc6 + d9), \\ & \quad -e^{-1t} dd8, -e^{-1t} (cc3 + dd5 - t22), -e^{1t} d8, -2 e^{\frac{31}{2}t} r19, -kl e^{-\frac{1}{2}t} (cc6 + d9 \\ & \quad \left. + 2 t22 - t36), -e^{21t} r19 (cc6 + d9) \right\} \end{aligned} \quad (51)$$

$$> sl2 := \text{solve} \left( \left\{ 2 kl e^{\frac{1}{2}t}, -2 k2 e^{-\frac{1}{2}t} \right\} \right)$$

$$sl2 := \{kl = 0, k2 = 0, t = t\}$$

(52)

(7D)

> restart : with(DifferentialGeometry) : with(LieAlgebras) : with(Tools) :  
Preferences("ShowFramePrompt",false) :

$$> L := \text{LieAlgebraData} \left( \left[ [X10, X01] = R, \right. \right.$$

$$[X10, Y10] = c1 X10 + c2 Y10 + t1 B,$$

$$[X10, Y01] = -dd1 X10 - X01 - dd2 Y10 - dd3 Y01 - dd4 Z + t4 B,$$

$$[X01, Y10] = -X10 - d1 X01 - d2 Y01 - d3 Y10 - d4 Z + t4 B,$$

$$[X01, Y01] = cc1 X01 + cc2 Y01 + t1 B,$$

$$[X10, Z] = -(cc3 + dd5) X10 - (cc4 + dd6) Y10 - Y01 - dd8 Z + t7 B,$$

$$[X01, Z] = -(c3 + d5) X01 - Y10 - (c4 + d6) Y01 - d8 Z + t7 B,$$

$$\begin{aligned}
[Y10, Y01] &= \exp(I t) Y10 - \exp(-I t) Y01 + t10 B, \\
[Y10, Z] &= -(c6 + dd9) Y10 - c7 Z + t13 B, \\
[Y01, Z] &= -(cc6 + d9) Y01 - cc7 Z + tt13 B, \\
[X10, R] &= r1 R + r2 X10 + r3 X01 + r4 Y10 + r5 Y01 + r6 Z + r7 B, \\
[X01, R] &= r10 R + r11 X10 + r12 X01 + r13 Y10 + r14 Y01 + r15 Z + r16 B, \\
[Y10, R] &= r19 R + r20 X10 + r21 X01 + r22 Y10 + r23 Y01 + r24 Z + r25 B, \\
[Y01, R] &= r28 R + r29 X10 + r30 X01 + r31 Y10 + r32 Y01 + r33 Z + r34 B, \\
[Z, R] &= r37 R + r38 X10 + r39 X01 + r40 Y10 + r41 Y01 + r42 Z + r43 B, \\
[B, R] &= r46 X10 + r47 X01 + r48 Y10 + r49 Y01 + r50 Z + r51 B, \\
[B, X10] &= \exp\left(\frac{I t}{2}\right) Y10 + t16 B, \\
[B, X01] &= \exp\left(-\frac{I t}{2}\right) Y01 + tt16 B, \\
[B, Y10] &= t19 B, [B, Y01] = tt19 B, \\
[B, Z] &= t22 B, \\
[R, X10, X01, Y10, Y01, Z, B], alg &):
\end{aligned}$$

> DGsetup(L) :

> JC := Query({a}, "Jacobi") : JC[1]; JCC := JC[2] : nops(JCC)

false

184

(53)

> JCC[1..16]

$$\left\{ e^{-\frac{1}{2}t} (c3 - cc6 + d5 - d9 - t22), -e^{-\frac{1}{2}t} cc7, -e^{-\frac{1}{2}t} (cc1 + tt19), -e^{\frac{1}{2}t} c7, -e^{\frac{1}{2}t} (c1 \right.$$

(54)

$$\left. + t19), -e^{\frac{1}{2}t} (c6 - cc3 - dd5 + dd9 + t22), -r12 - r2, e^{-1t} cc7 - e^{1t} c7, -e^{-1t} r28 \right.$$

$$\left. + e^{1t} r19, e^{-1t} tt19 - e^{1t} t19, -e^{-\frac{1}{2}t} r28 + r46, -e^{\frac{1}{2}t} r19 - r47, -c7 + e^{-1t} - c1, \right.$$

$$\left. -cc1 + dd1 - r28, -cc7 + e^{1t} - cc1, d1 - c1 - r19 \right\}$$

> sll := solve(JCC[1..16]) : JCC1 := simplify(eval(JCC, sll)) :

> JCC1[1..16]

$$\left\{ 0, r19 \left( e^{\frac{31}{2}t} r19 + 3 e^{\frac{1}{2}t} \right), (cc6 + d9) e^{1t}, e^{-1t} (c2 - t16), e^{-1t} (cc3 + dd5 - t22), \right. \quad (55)$$

$$e^{1t} (cc2 - tt16), e^{\frac{1}{2}t} r19 (cc6 + d9 - r37 + 2 t22), -r19 \left( e^{\frac{51}{2}t} r19 + 3 e^{\frac{31}{2}t} \right),$$

$$-r19 (cc3 + dd5 - t22), -(cc6 + d9) e^{1t}, -(e^{21t} r19 + e^{1t}) (cc6 + d9), -(e^{-1t}$$

$$+ r19) (cc3 + dd5 - t22), -e^{-1t} dd8, -e^{-1t} (cc3 + dd5 - t22), -e^{1t} d8, 2 e^{\frac{1}{2}t} r19 \left. \right\}$$

$$\begin{aligned} &> sl2 := solve \left( \left\{ (cc6 + d9) e^{1t}, e^{-1t} (c2 - t16), e^{-1t} (cc3 + dd5 - t22), e^{1t} (cc2 - tt16), \right. \right. \\ &\quad \left. \left. -(cc6 + d9) e^{1t}, -e^{-1t} dd8, -e^{-1t} (cc3 + dd5 - t22), -e^{1t} d8, 2 e^{\frac{1}{2}t} r19 \right\} \right) : JCC2 := \\ &\quad simplify(eval(JCC1, sl2)) : \end{aligned}$$

$$\begin{aligned} &> JCC2[1..10] \\ &\quad \{-3, 0, 3, r50 (r37 - t22), r50 e^{-1t}, r50 e^{t1}, -d4 t22, -dd4 t22, -3 e^{-1t}, 3 e^{t1}\} \end{aligned} \quad (56)$$

>  
The same conclusion: in all cases of filtered deformation of the 6D orbit on 3ndg 7D CR of type dim (U\_L)=1, dim(U\_K)=3, the ideal of Jacobi identity relations contains element 1, hence the algebra is not realizable.
