# Supplementary material for: On 3-nondegenerate CR manifolds in dimension 7 (II): the intransitive case
Source: arXiv:2308.02841 ancillary file (2025-09-15)
Supplement: Supplementary file 2 [file 7D3ndg_II2.pdf]

Maple accompanying the paper "On 3-nondegenerate CR manifolds in dimension 7 (II): the intransitive case" by Boris Kruglikov and Andrea Santi

>

We compute the Tanaka prolongation of the 5D orbit on 3ndg 7D CR of type  $\dim(U_L)=0, \dim(U_K)=2, \dim(U_D^J)=2$  with 1D structure reduction

> *restart* : with (DifferentialGeometry) : with (LieAlgebras) : with (GroupActions) : with (Tools) :  
Preferences ("ShowFramePrompt",false) :

> *L* := LieAlgebraData ([ [X10, X01] = R], [R, X10, X01, Y10, Y01], alg, grading = [-2, -1, -1, -1, -1]) :

> DGsetup(L) :

> infolevel[TanakaProlongation] := 2 :

> prL0 := TanakaProlongation(alg, 1, pralg0)

m:

[e1], [e2, e3, e4, e5]  
[-2, -1]

g^(0):

[e1], [e2, e3, e4, e5], [e6, e7, e8, e9, e10, e11, e12, e13, e14, e15, e16, e17]  
[-2, -1, 0]

prL0 := [[e1, e6] = -e1, [e2, e3] = e1, [e2, e7] = -e2, [e2, e9] = -e3, [e2, e10] = -e4, [e2, e14] = -e5, [e3, e6] = -e3, [e3, e7] = e3, [e3, e8] = -e2, [e3, e11] = -e4, [e3, e15] = -e5, [e4, e12] = -e4, [e4, e16] = -e5, [e5, e13] = -e4, [e5, e17] = -e5, [e6, e8] = -e8, [e6, e9] = e9, [e6, e11] = -e11, [e6, e15] = -e15, [e7, e8] = 2 e8, [e7, e9] = -2 e9, [e7, e10] = -e10, [e7, e11] = e11, [e7, e14] = -e14, [e7, e15] = e15, [e8, e9] = e7, [e8, e10] = -e11, [e8, e14] = -e15, [e9, e11] = -e10, [e9, e15] = -e14, [e10, e12] = -e10, [e10, e16] = -e14, [e11, e12] = -e11, [e11, e16] = -e15, [e12, e13] = e13, [e12, e16] = -e16, [e13, e14] = e10, [e13, e15] = e11, [e13, e16] = e12 - e17, [e13, e17] = e13, [e14, e17] = -e14, [e15, e17] = -e15, [e16, e17] = -e16] (1)

> DGsetup(prL0) :

> for j to 5 do print(LieBracket(e||j, add((a||i)·(e||i), i = 6..17))) :od  
-a6 e1

-a7 e2 - a9 e3 - a10 e4 - a14 e5  
-a8 e2 - (-a7 + a6) e3 - a11 e4 - a15 e5  
-a12 e4 - a16 e5  
-a13 e4 - a17 e5 (2)

First we consider scaling extension, its positive prolongation is trivial

> S := -2 e6 - e7 :  
seq(LieBracket(S, e||i), i = 1..5)  
-2 e1, -e2, -e3, 0 e1, 0 e1 (3)

> L1 := ChangeGradedComponent(pralg0, [ 0 = [S]], alg1)  
L1 := [[e1, e6] = 2 e1, [e2, e3] = e1, [e2, e6] = e2, [e3, e6] = e3] (4)

> DGsetup(L1) :

>  $LL := \text{TanakaProlongation}(\text{alg1}, 4, \text{pralg1})$

m:

$[[e1], [e2, e3, e4, e5], [e6]]$   
 $[-2, -1, 0]$

$$LL := [[e1, e6] = 2 e1, [e2, e3] = e1, [e2, e6] = e2, [e3, e6] = e3] \quad (5)$$

Next we consider  $\beta$ -structure group reduction (with freedom for  $\beta$  reduced from 1 complex to 1 real dimension). Here the positive prolongation has 2 dimensions (below  $b=i*r*\exp(i*\psi)$ ,  $bb=-i*r*\exp(-i*\psi)$ )

>  $\text{ChangeFrame}(\text{pralg0}) :$

>  $B := b e10 + bb e15 :$

$\text{seq}(\text{LieBracket}(B, e \parallel i), i = 1 \dots 5)$

$$0 e1, b e4, bb e5, 0 e1, 0 e1 \quad (6)$$

>  $L1 := \text{ChangeGradedComponent}(\text{pralg0}, [0 = [B]], \text{alg1})$

$$L1 := [[e2, e3] = e1, [e2, e6] = -b e4, [e3, e6] = -bb e5] \quad (7)$$

>  $\text{DGsetup}(L1) :$

>  $LL := \text{TanakaProlongation}(\text{alg1}, 4, \text{pralg1})$

m:

$[[e1], [e2, e3, e4, e5], [e6]]$   
 $[-2, -1, 0]$

$g^{(1)}:$

$[[e1], [e2, e3, e4, e5], [e6], [e7, e8]]$   
 $[-2, -1, 0, 1]$

$$LL := \left[ [e1, e7] = -e4, [e1, e8] = -e5, [e2, e3] = e1, [e2, e6] = -b e4, [e2, e8] = -\frac{e6}{bb}, [e3, e6] = -bb e5, [e3, e7] = \frac{e6}{b} \right] \quad (8)$$

So we have to setup the structure relations and check Jacobi to exclude 8D and 7D cases. We start with 8D

(below  $c1=b$ ,  $c2=bb$ ,  $m=s1+i*s2$ ,  $mm=s1-i*s2$ )

>  $\text{restart} : \text{with}(\text{DifferentialGeometry}) : \text{with}(\text{LieAlgebras}) : \text{with}(\text{GroupActions}) : \text{with}(\text{Tools}) :$   
 $\text{Preferences}(\text{"ShowFramePrompt"}, \text{'false'}) :$

$$\begin{aligned} > L := \text{LieAlgebraData} \left( \left[ [X10, X01] = R, [X10, Y10] = Y01 + b1 X10 + b2 Y10 + r1 B \right. \right. \\ &\quad + r2 B10 + r3 B01, [X10, Y01] = m X01 + a1 X10 + a2 Y10 + a3 Y01 + r4 B + r5 B10 \\ &\quad + r6 B01, [X10, B] = -c1 Y10 + t1 B + t2 B10 + t3 B01, [X10, B10] = t4 B10 + t5 B01, \\ &\quad [X10, B01] = -\frac{1}{c2} B + t6 B10 + t7 B01, [X01, Y10] = mm X10 + aa1 X01 + aa2 Y01 \\ &\quad + aa3 Y10 + r7 B + r8 B10 + r9 B01, [X01, Y01] = Y10 + bb1 X01 + bb2 Y01 + r10 B \\ &\quad + r11 B10 + r12 B01, [X01, B] = -c2 Y01 + t8 B + t9 B10 + t10 B01, [X01, B10] \\ &\quad \left. = \frac{1}{c1} B + t11 B10 + t12 B01, [X01, B01] = t13 B10 + t14 B01, [Y10, Y01] = k Y10 \right] \end{aligned}$$

$-kk Y01 + r13 B + r14 B10 + r15 B01, [Y10, B] = t15 B + t16 B10 + t17 B01, [Y10, B10] = t18 B10 + t19 B01, [Y10, B01] = t20 B10 + t21 B01, [Y01, B] = t22 B + t23 B10 + t24 B01, [Y01, B10] = t25 B10 + t26 B01, [Y01, B01] = t27 B10 + t28 B01, [R, X10] = s1 R + s2 X10 + s3 X01 + s4 Y10 + s5 Y01 + s6 B + s7 B10 + s8 B01, [R, X01] = s9 R + s10 X10 + s11 X01 + s12 Y10 + s13 Y01 + s14 B + s15 B10 + s16 B01, [R, Y10] = s17 R + s18 X10 + s19 X01 + s20 Y10 + s21 Y01 + s22 B + s23 B10 + s24 B01, [R, Y01] = s25 R + s26 X10 + s27 X01 + s28 Y10 + s29 Y01 + s30 B + s31 B10 + s32 B01, [R, B] = s33 X10 + s34 X01 + s35 Y10 + s36 Y01 + s37 B + s38 B10 + s39 B01, [R, B10] = -Y10 + s40 B + s41 B10 + s42 B01, [R, B01] = -Y01 + s43 B + s44 B10 + s45 B01, [R, X10, X01, Y10, Y01, B, B10, B01], Alg) :$

> DGsetup(L) :

> Q := Query({a}, "Jacobi")[2] :

We are going to simplify this long system of polynomial equations, assuming c1,c2 nonzero (which are b,bb, i.e. expressed through  $\beta$  and its conjugate), also m,mm nonzero (by the initial conditions and nondegeneracy)

> Q[1..7]

$$\left\{ t19, t27, \frac{t19}{c2}, \frac{-t18 + t15 + aa1}{c1}, \frac{-t25 + t22 + bb1}{c1}, \frac{c1 t15 + s34}{c1}, \frac{c2 t22 - s33}{c2} \right\} \quad (9)$$

> S11 := solve(Q[1..7])

S11 := {aa1 = t18 - t15, bb1 = t25 - t22, c1 = c1, c2 = c2, s33 = c2 t22, s34 = -c1 t15, t15 = t15, t18 = t18, t19 = 0, t22 = t22, t25 = t25, t27 = 0} (10)

> QQ := simplify(eval(Q, S11)) :

> S12 := solve({(s17 - t15), (-a1 + k + t22), (s25 - t22), (2 t22 - t25), (kk + 2 t15 - t18), (b1 + kk + t15 - t18), (a1 - k + t22 - t25), -b1, -t18, -t20, -t21, -(b1 - t15), -t25, -t26, -t28, -a1 + t22, s11 + s2, t13 - 1, -t18 + 2 t15, t18 - s17, t20 - k, -t25 + t22, t25 - t20, t26 - kk, t26 - t21, t28 - s25, t5 - 1})

S12 := {a1 = 0, b1 = 0, k = 0, kk = 0, s11 = -s2, s17 = 0, s2 = s2, s25 = 0, t13 = 1, t15 = 0, t18 = 0, t20 = 0, t21 = 0, t22 = 0, t25 = 0, t26 = 0, t28 = 0, t5 = 1} (11)

> QQ := simplify(eval(QQ, S12)) :

> QQ[1..20]

$\left\{ 0, s19, t16, t17, t23, t24, a2 mm, c1 s18, c2 s27, \frac{m}{c1}, m c2, m mm, m s18, m t11, m t12, mm t6, mm t7, \frac{s19}{c1}, \frac{t17}{c2}, \frac{t23}{c1} \right\}$  (12)

Contradiction with  $m \neq 0, mm \neq 0$ . Thus 8D is not possible. Consider reduction of g[1] to 1D, hence the algebra to 7D

> restart : with(DifferentialGeometry) : with(LieAlgebras) : with(GroupActions) : with(Tools) : Preferences("ShowFramePrompt", false) :

> L := LieAlgebraData( $\left[ \begin{aligned} &[X10, X01] = R, [X10, Y10] = Y01 + b1 X10 + b2 Y10 + r1 B \\ &+ r2 B11, [X10, Y01] = m X01 + a1 X10 + a2 Y10 + a3 Y01 + r4 B + r5 B11, [X10, B] = \\ &-c1 Y10 + t1 B + t2 B11, [X10, B11] = \frac{p2}{c2} B + t6 B11, [X01, Y10] = mm X10 + aa1 X01 \end{aligned} \right.$ )

$$\begin{aligned}
& + aa2 Y01 + aa3 Y10 + r7 B + r8 B11, [X01, Y01] = Y10 + bb1 X01 + bb2 Y01 + r10 B \\
& + r11 B11, [X01, B] = -c2 Y01 + t8 B + t9 B11, [X01, B11] = -\frac{p1}{c1} B + t11 B11, [Y10, \\
& Y01] = k Y10 - kk Y01 + r13 B + r14 B11, [Y10, B] = t15 B + t16 B11, [Y10, B11] \\
& = t18 B11, [Y01, B] = t22 B + t23 B11, [Y01, B11] = t25 B11, [R, X10] = s1 R + s2 X10 \\
& + s3 X01 + s4 Y10 + s5 Y01 + s6 B + s7 B11, [R, X01] = s9 R + s10 X10 + s11 X01 \\
& + s12 Y10 + s13 Y01 + s14 B + s15 B11, [R, Y10] = s17 R + s18 X10 + s19 X01 \\
& + s20 Y10 + s21 Y01 + s22 B + s23 B11, [R, Y01] = s25 R + s26 X10 + s27 X01 \\
& + s28 Y10 + s29 Y01 + s30 B + s31 B11, [R, B] = s33 X10 + s34 X01 + s35 Y10 \\
& + s36 Y01 + s37 B + s38 B11, [R, B11] = p1 Y10 + p2 Y01 + s40 B + s41 B11 \Big], [R, \\
& X10, X01, Y10, Y01, B, B11], Alg \Big):
\end{aligned}$$

> DGsetup(L) :

> Q := Query({a}, "Jacobi")[2] :

We are going to simplify this long system of polynomial equations, assuming c1,c2 nonzero, p1 or p2 nonzero, and also m,mm nonzero (by the initial conditions and nondegeneracy).

In fact, to simplify computation, we may assume by symmetry that p1=1, p2=p (any)

> restart : with(DifferentialGeometry) : with(LieAlgebras) : with(GroupActions) : with(Tools) :  
Preferences("ShowFramePrompt",false) :

$$\begin{aligned}
& > L := LieAlgebraData \left( \left[ [X10, X01] = R, [X10, Y10] = Y01 + b1 X10 + b2 Y10 + r1 B \right. \right. \\
& \quad + r2 B11, [X10, Y01] = m X01 + a1 X10 + a2 Y10 + a3 Y01 + r4 B + r5 B11, [X10, B] = \\
& \quad -c1 Y10 + t1 B + t2 B11, [X10, B11] = \frac{p}{c2} B + t6 B11, [X01, Y10] = mm X10 + aa1 X01 \\
& \quad + aa2 Y01 + aa3 Y10 + r7 B + r8 B11, [X01, Y01] = Y10 + bb1 X01 + bb2 Y01 + r10 B \\
& \quad + r11 B11, [X01, B] = -c2 Y01 + t8 B + t9 B11, [X01, B11] = -\frac{1}{c1} B + t11 B11, [Y10, \\
& \quad Y01] = k Y10 - kk Y01 + r13 B + r14 B11, [Y10, B] = t15 B + t16 B11, [Y10, B11] \\
& \quad = t18 B11, [Y01, B] = t22 B + t23 B11, [Y01, B11] = t25 B11, [R, X10] = s1 R + s2 X10 \\
& \quad + s3 X01 + s4 Y10 + s5 Y01 + s6 B + s7 B11, [R, X01] = s9 R + s10 X10 + s11 X01 \\
& \quad + s12 Y10 + s13 Y01 + s14 B + s15 B11, [R, Y10] = s17 R + s18 X10 + s19 X01
\end{aligned}$$

$$\begin{aligned}
& + s_{20} Y_{10} + s_{21} Y_{01} + s_{22} B + s_{23} B_{11}, [R, Y_{01}] = s_{25} R + s_{26} X_{10} + s_{27} X_{01} \\
& + s_{28} Y_{10} + s_{29} Y_{01} + s_{30} B + s_{31} B_{11}, [R, B] = s_{33} X_{10} + s_{34} X_{01} + s_{35} Y_{10} \\
& + s_{36} Y_{01} + s_{37} B + s_{38} B_{11}, [R, B_{11}] = Y_{10} + p Y_{01} + s_{40} B + s_{41} B_{11} \Big], [R, X_{10}, \\
& X_{01}, Y_{10}, Y_{01}, B, B_{11}], Alg \Big) :
\end{aligned}$$

$$\begin{aligned}
& \triangleright DGsetup(L) : \\
& \triangleright Q := Query(\{a\}, "Jacobi")[2] : \\
& \triangleright Q[1..50] : \\
& \triangleright SII := solve(\{c1\ mm + s33, -t18, -t25, s11 + s2, -aa1 - b1 + s17, -bb1 - a1 + s25, -t25 \\
& \quad - k + s25, -b1\ c1 + t15\ c1, -bb1\ c2 + c2\ t22, c1\ s17 + s34, p\ (-t18 + b1 + t15), \\
& \quad p\ (c2\ m - s34), c2\ s25 - s33, -c1\ mm - c2\ k, -c1\ kk - c2\ m, -k\ s17 + kk\ s25, k\ t15 \\
& \quad - kk\ t22, k\ t18 - kk\ t25\}) : nops(\{SII\})
\end{aligned} \tag{13}$$

$$\begin{aligned}
& \triangleright seq(eval([c1, c2, m, mm], SII[k]), k = 1..17) \\
& \left[ c1, c2, m, -\frac{c2\ s25}{c1} \right], [c1, c2, 0, 0], [c1, c2, m, 0], [c1, 0, m, 0], \left[ c1, c2, 0, -\frac{c2\ s25}{c1} \right], \left[ c1, \right. \\
& \quad \left. c2, m, -\frac{c2\ s25}{c1} \right], [c1, 0, m, 0], [0, c2, 0, mm], [0, c2, 0, mm], [0, c2, 0, mm], [0, c2, 0, \\
& \quad mm], [0, 0, m, mm], [0, 0, m, mm], [0, 0, m, mm], [0, 0, m, mm], [0, 0, m, mm], [0, 0, m, \\
& \quad mm]
\end{aligned} \tag{14}$$

$$\begin{aligned}
& \triangleright \# SII[1]; SII[6] \\
& \left\{ a1 = -t22 + s25, aa1 = -\frac{c2\ m\ (-t22 + s25)}{c1\ s25}, b1 = -\frac{c2\ m\ t22}{c1\ s25}, bb1 = t22, c1 = c1, c2 \right. \\
& \quad = c2, k = s25, kk = -\frac{c2\ m}{c1}, m = m, mm = -\frac{c2\ s25}{c1}, p = 0, s11 = -s2, s17 = -\frac{c2\ m}{c1}, s2 \\
& \quad = s2, s25 = s25, s33 = c2\ s25, s34 = c2\ m, t15 = -\frac{c2\ m\ t22}{c1\ s25}, t18 = 0, t22 = t22, t25 = 0 \Big\} \\
& \left\{ a1 = s25, aa1 = -\frac{c2\ m}{c1}, b1 = 0, bb1 = 0, c1 = c1, c2 = c2, k = s25, kk = -\frac{c2\ m}{c1}, m = m, mm \right. \\
& \quad = -\frac{c2\ s25}{c1}, p = p, s11 = -s2, s17 = -\frac{c2\ m}{c1}, s2 = s2, s25 = s25, s33 = c2\ s25, s34 \\
& \quad = c2\ m, t15 = 0, t18 = 0, t22 = 0, t25 = 0 \Big\}
\end{aligned} \tag{15}$$

$$\begin{aligned}
& \triangleright QQ1 := simplify(eval(Q, SII[1])) : \\
& \triangleright QQ1[1..5] \\
& \left\{ 0, 1, c2\ (-t22 + 3\ s25), \frac{((s25 + t22)\ s40 - r13)\ c1 - s27}{c1}, \right. \\
& \quad \left. \frac{((s1 + t1 - t6)\ s40 + r1)\ c1 - s3}{c1} \right\}
\end{aligned} \tag{16}$$

> QQ2 := simplify(eval(Q, SI[6])) :

> QQ2[51..100]

$$\left\{ \frac{1}{cl} (-s_{22} cl^2 + (s_{21} a_2 + s_3 aa_3 + s_2 b_2 - r_1 s_{35} + s_1 s_{20} - s_5 s_{25} - r_2 - s_{28}) cl \right. \quad (17)$$

$$+ m c_2 s_4), \frac{1}{cl} (((-tl_1 + aa_3 + bb_2) r_{14} + r_{10} tl_6 - r_{13} t_9 - s_{25} r_8 - r_7 t_{23}) cl$$

$$- 2 m r_{11} c_2 - c_2 r_5 s_{25}), \frac{1}{cl} (((t_8 - aa_3 + s_9) s_{22} + (s_{20} - s_{37} - s_2) r_7$$

$$- aa_2 s_{30} + r_{10} s_{21} - r_{13} s_{13} + r_1 s_{10} - s_{40} r_8) cl + (2 m s_{14} + s_{25} s_6) c_2$$

$$- s_{23}), \frac{1}{cl} ((-aa_2 s_{28} - s_2 aa_3 + s_{10} b_2 - r_7 s_{35} - s_{13} s_{25} + s_9 s_{20} - r_8 + s_{21}) cl$$

$$+ 2 c_2 m s_{12} + s_4 c_2 s_{25}),$$

$$\frac{((-t_8 + aa_3 + bb_2) r_{13} - s_{25} r_7) cl - 2 c_2 m r_{10} - c_2 s_{25} r_4 + r_{14}}{cl},$$

$$\frac{-cl p s_{25} + c_2 m}{cl^2}, \frac{cl p s_{25} - c_2 m}{cl}, \frac{cl s_{25} tl_6 + c_2 m t_{23}}{cl},$$

$$\frac{-a_2 c_2 s_{25} + bb_2 cl s_{25} - 2 c_2 m}{cl}, \frac{-c_2 m tl_1 - c_2 s_{25} t_6 - tl_6}{cl},$$

$$\frac{c_2 m tl_1 + c_2 s_{25} t_6 + t_{23} p}{c_2}, \frac{c_2 (((s_9 - t_8) m + s_{27}) cl - m s_{35})}{cl}, \frac{p tl_6}{c_2},$$

$$\frac{(c_2 s_{40} + p (t_8 - tl_1)) cl + (tl - t_6) c_2}{cl c_2}, \frac{(((s_9 - t_8) s_{25} + s_{26}) cl - s_{25} s_{35}) c_2}{cl},$$

$$\frac{((p r_4 + (s_1 + tl - t_6) s_{40} + r_1) c_2 - p (s_{37} - s_{41} - s_2)) cl - s_3 c_2}{cl c_2},$$

$$\frac{(((a_3 + b_2 - tl) r_{13} - m r_7 - 2 s_{25} r_1) c_2 - p r_{14}) cl - c_2^2 m r_4}{cl c_2},$$

$$\frac{(((a_3 - tl) r_{10} + (-bb_2 + t_8) r_4 + a_2 r_7 + s_{30} - r_1) c_2 - r_{11} p) cl - c_2 r_5}{cl c_2},$$

$$\frac{(((t_8 - aa_3) r_1 + (b_2 - tl) r_7 - r_4 aa_2 + r_{10} + s_{22}) c_2 - r_8 p) cl - r_2 c_2}{cl c_2},$$

$$\frac{1}{cl c_2} (((tl + s_1) s_{14} + (-s_9 - t_8) s_6 - r_{10} s_5 + s_{12} r_1 + s_{13} r_4 - r_7 s_4) c_2$$

$$\begin{aligned}
& + p s15) c1 + s7 c2), \frac{1}{c1 c2} ( ((t1 - b2 + s1) s22 + (s2 + s20 - s37) r1 + s3 r7 \\
& - s5 r13 + r4 s21 - r2 s40 - s30) c2 + s23 p) c1 + c2^2 m s6), \\
& \frac{((s25 s40 - r13) c2 + p s26) c1 - c2 s27}{c1 c2}, \\
& \frac{(((s9 + t8 - t11) s40 + p r10 + r7) c1 + s37 - s41 + s2) c2 + c1 p s10}{c1 c2}, \\
& \frac{(c1 s41 + t2) c2 + c1 p t9}{c1 c2}, \frac{-c1^2 c2 r7 + (c2^2 r4 + s37 c2 - p t9) c1 - t2 c2}{c1 c2}, \\
& \frac{-c2^2 m s40 + (c1 p r13 - s19) c2 + c1 p s18}{c1 c2}, \frac{c1 p s25 - c2 m}{c1 c2}, 3 c2 m, 3 c2 s25, \\
& -\frac{t23}{c1}, -\frac{p t16}{c2}, ((s1 - t1) c2 + s36) m + c1 s19, ((s1 - t1) c2 + s36) s25 + c1 s18, \\
& (b2 + t1 - t6) t16 + t23, (t8 + bb2 - t11) t23 + t16, (-aa2 m - s19 - s25) c2 - p t16, \\
& (a3 - t1) c2 - aa2 c1 + s36, (-b2 + s1) s19 + (-c2 r1 + s21) m - s27, (t8 - aa3) c1 \\
& + a2 c2 + s35, (-a2 s25 - m) c2 - c1 s26 - t23, (b2 + s1 - t1) s35 + (s20 - s37 \\
& - s2) c1 + a2 s36 - t2, (s9 - t8 + bb2) s36 + (-s37 + s2 + s29) c2 - p t9 + aa2 s35, \\
& (-c2 r4 - s2 + s29) s25 + (-a3 + s1) s26 - m s10 - a2 s18, (-c2 r4 + 2 s2 + s29) m \\
& + (-a3 + s1) s27 - 2 s25 s3 - a2 s19, (-a3 + b2) aa2 - c2 r1 - aa3 + bb2 + s21, \\
& (a3 + s1) s13 + (-s9 - bb2) s5 + s6 c2 - aa2 s4 + s12, (aa3 - bb2) a2 + r10 c1 + a3 \\
& - b2 + s28, (b2 + s1) s12 + (-s9 - aa3) s4 + a2 s13 - c1 s14 - s5, (t11 - t8) t2 \\
& + (t1 - t6) t9 - c1 r8 + c2 r5 + s38, (a3 + s1 - t1) s36 - p t2 + c1 s21 - s3 c2 + s35\}
\end{aligned}$$

$$\begin{aligned}
> Sl2 := solve(\{t23, (1 + (a3 + s1 - t6) p) c2 - p s36, (s19 - s25) c1 + m b2 c2, c1 p s25 \\
& - c2 m, m, s25, -t23, -p t16\}) : nops(\{Sl2\}) \\
& \quad \quad \quad 4 \tag{18}
\end{aligned}$$

$$\begin{aligned}
> seq(eval([c1, c2, m, mm], Sl2[k]), k=1..4) \\
& \quad \quad \quad [0, 0, 0, mm], [c1, 0, 0, mm], [0, c2, 0, mm], [c1, c2, 0, mm] \tag{19}
\end{aligned}$$

Thus 7D case is also non-realizable!
