# Supplementary material for: On 3-nondegenerate CR manifolds in dimension 7 (II): the intransitive case
Source: arXiv:2308.02841 ancillary file (2025-09-15)
Supplement: Supplementary file 3 [file 7D3ndg_II3.pdf]

Maple accompanying the paper "On 3-nondegenerate CR manifolds in dimension 7 (II): the intransitive case" by Boris Kruglikov and Andrea Santi

>

In this worksheet we study 3-nondegenerate 7D CR manifold M7 of the tube type over cone over tangent to a nondegenerate curve in P3 with 6D affine symmetry algebra

> with(DifferentialGeometry) : with(LieAlgebras) : with(Tensor) : with(Tools) :  
Preferences("ShowFramePrompt",false) :

>

We parametrize a homogeneous curve in P3 and its tangent cone in computationally convenient way.  
Preparation to compute symmetries.

> DGsetup([x0, x1, x2, x3], M) :

> X := evalDG(add(add((a || i || j) · (x || i) D\_x || j, i = 0..3), j = 0..3)) :

> solve({coeffs(expand(eval(LieDerivative(X, x0 x2 - x1^2), {x0 = 1, x1 = q, x2 = q^2, x3 = q^3})), {q}), coeffs(expand(eval(LieDerivative(X, x0^2 x3 - x1^3), {x0 = 1, x1 = q, x2 = q^2, x3 = q^3})), {q})), eval(Matrix([ [a00, a01, a02, a03], [a10, a11, a12, a13], [a20, a21, a22, a23], [a30, a31, a32, a33]]), %)  
{a00 = 3 a22 - 2 a33, a01 = a01, a02 = 0, a03 = 0, a10 = 3 a32, a11 = 2 a22 - a33, a12 = 2 a01, a13 = 0, a20 = 0, a21 = 2 a32, a22 = a22, a23 = 3 a01, a30 = 0, a31 = 0, a32 = a32, a33 = a33}

$$\begin{bmatrix} 3 a_{22} - 2 a_{33} & a_{01} & 0 & 0 \\ 3 a_{32} & 2 a_{22} - a_{33} & 2 a_{01} & 0 \\ 0 & 2 a_{32} & a_{22} & 3 a_{01} \\ 0 & 0 & a_{32} & a_{33} \end{bmatrix} \quad (1)$$

> # simplify(expand(eval(LieDerivative(X, x0^{m-1} x2 - x1^m), {x0 = 1, x1 = q, x2 = q^m, x3 = q^n}))) assuming m < n

# simplify(expand(eval(LieDerivative(X, x0^{n-1} x3 - x1^n), {x0 = 1, x1 = q, x2 = q^m, x3 = q^n}))) assuming m < n

> X0 := eval(add((a || i) · (x || i) D\_x || i, i = 0..3), {a0 = λ, a1 = μ, a2 = m μ - (m - 1) λ, a3 = n μ - (n - 1) λ}) :  
expand(eval([LieDerivative(X0, x0^{m-1} x2 - x1^m), LieDerivative(X0, x0^{n-1} x3 - x1^n)], {x0 = 1, x1 = q, x2 = q^m, x3 = q^n}))

$$[0, 0] \quad (2)$$

> v := simplify(λ + μ + (m μ - (m - 1) λ) + (n μ - (n - 1) λ)); solve({λ - \frac{v}{4} = -3 a, μ - \frac{v}{4} = -a, m μ - (m - 1) λ - \frac{v}{4} = a, n μ - (n - 1) λ - \frac{v}{4} = 3 a, a ≠ 0})

$$v := (-m - n + 3) λ + μ (m + n + 1)$$

$$\left\{ a = -\frac{λ}{2} + \frac{μ}{2}, λ = λ, m = 2, μ = μ, n = 3 \right\} \quad (3)$$

$$\begin{aligned}
& \text{> } X0 := \text{eval}(\text{add}((a||i) \cdot (x||i) D\_x||i, i=0..3), \{a0=\lambda, a1=\lambda+\mu, a2=\lambda+m\mu, a3=\lambda \\
& \quad + n\mu\}) : \\
& \text{expand}(\text{eval}([LieDerivative(X0, x0^{m-1}x2 - x1^m), LieDerivative(X0, x0^{n-1}x3 - x1^n)], \{x0 \\
& \quad = 1, x1=q, x2=q^m, x3=q^n\})) \\
& \qquad \qquad \qquad [0, 0] \tag{4}
\end{aligned}$$

$$\begin{aligned}
& \text{> } \text{solve}(\{\text{coeffs}(\text{expand}(\text{eval}(LieDerivative(X, x0x2 - x1^2), \{x0=1, x1=q, x2=q^2, x3 \\
& \quad = q^4\})), \{q\}), \text{coeffs}(\text{expand}(\text{eval}(LieDerivative(X, x0^3x3 - x1^4), \{x0=1, x1=q, x2 \\
& \quad = q^2, x3=q^4\})), \{q\})\}); \text{eval}(\text{Matrix}([a00, a01, a02, a03], [a10, a11, a12, a13], [a20, \\
& \quad a21, a22, a23], [a30, a31, a32, a33])), \%) \\
& \{a00=2a11 - a22, a01=0, a02=0, a03=0, a10=0, a11=a11, a12=0, a13=0, a20=0, a21 \\
& \quad = 0, a22=a22, a23=0, a30=0, a31=0, a32=0, a33=-2a11 + 3a22\} \\
& \quad \quad \quad \begin{bmatrix} 2a11 - a22 & 0 & 0 & 0 \\ 0 & a11 & 0 & 0 \\ 0 & 0 & a22 & 0 \\ 0 & 0 & 0 & -2a11 + 3a22 \end{bmatrix} \tag{5}
\end{aligned}$$

$$\begin{aligned}
& \text{> } \text{eliminate}(\{x1=q+t, x2=q^2+2qt, x3=q^4+4q^3t\}, \{q, t\})[2] \\
& \quad \{16x1^4x3 - 8x1^2x2^3 - 24x1^2x2x3 + 9x2^4 + 6x2^2x3 + x3^2\} \tag{6}
\end{aligned}$$

$$\begin{aligned}
& \text{> } \text{sxr} := \{x0=r^4, x1=r^3 \cdot (q+t), x2=r^2 \cdot (q^2+2qt), x3=q^4+4q^3t\} : \\
& \text{> } \# \text{eliminate}(\text{sxr}, \{r, q, t\})[1][2] \\
& \text{> } \text{simplify}(\text{eval}(16x1^4x3 - 8x1^2x2^3 - 24x0x1^2x2x3 + 9x0x2^4 + 6x0^2x2^2x3 + x0^3x3^2, \\
& \quad \text{sxr})) \\
& \qquad \qquad \qquad 0 \tag{7}
\end{aligned}$$

$$\begin{aligned}
& \text{> } \text{convert}(\text{solve}(\text{sxr}[1..3], \{r, q, t\}), 'radical') \\
& \quad \left\{ q = \frac{x0^{1/4}x1 + \sqrt{\sqrt{x0}x1^2 - x0^{3/2}x2}}{x0}, r = x0^{1/4}, t = -\frac{\sqrt{\sqrt{x0}x1^2 - x0^{3/2}x2}}{x0} \right\} \tag{8}
\end{aligned}$$

$$\begin{aligned}
& \text{> } \text{srx} := \left\{ r = x0^{1/4}, q = \frac{x1 + \sqrt{x1^2 - x0x2}}{x0^{3/4}}, t = -\frac{\sqrt{x1^2 - x0x2}}{x0^{3/4}} \right\} : \text{simplify}(\text{subs}(\text{srx}, \text{sxr})) \\
& \quad \left\{ x0=x0, x1=x1, x2=x2, x3 = \frac{(x1 - 3\sqrt{-x2x0 + x1^2})(x1 + \sqrt{-x2x0 + x1^2})^3}{x0^3} \right\} \tag{9}
\end{aligned}$$

> Let us check 3-nondegeneracy of TRNC as 7D CR manifold Sigma3(x)xR4(y).

$$\begin{aligned}
& \text{> } \text{DGsetup}([x0, x1, x2, x3, y0, y1, y2, y3], R8) : \\
& \text{> } X1 := \text{evalDG}(\text{eval}(4r^3D\_x0 + 3r^2 \cdot (q+t)D\_x1 + 2r \cdot (q^2+2qt)D\_x2, \text{srx})): X2 := \\
& \quad \text{evalDG}(\text{eval}(r^3D\_x1 + 2r^2 \cdot (q+t)D\_x2 + 4q^2 \cdot (q+3t)D\_x3, \text{srx})): X3 := \\
& \quad \text{evalDG}(\text{eval}(r^3D\_x1 + 2r^2qD\_x2 + 4q^3D\_x3, \text{srx})): \\
& Y1 := \text{evalDG}(\text{eval}(4r^3D\_y0 + 3r^2 \cdot (q+t)D\_y1 + 2r \cdot (q^2+2qt)D\_y2, \text{srx})): Y2 := \\
& \quad \text{evalDG}(\text{eval}(r^3D\_y1 + 2r^2 \cdot (q+t)D\_y2 + 4q^2 \cdot (q+3t)D\_y3, \text{srx})): Y3 :=
\end{aligned}$$

$$\begin{aligned}
& evalDG( eval( r^3 D_y1 + 2 r^2 q D_y2 + 4 q^3 D_y3, srx ) ) : \\
zz1 &:= evalDG\left(\frac{X1 - I Y1}{2}\right) : ZZ1 := evalDG\left(\frac{X1 + I Y1}{2}\right) : zz2 := \\
& evalDG\left(\frac{X2 - I Y2}{2}\right) : ZZ2 := evalDG\left(\frac{X2 + I Y2}{2}\right) : zz3 := evalDG\left(\frac{X3 - I Y3}{2}\right) : \\
ZZ3 &:= evalDG\left(\frac{X3 + I Y3}{2}\right) :
\end{aligned}$$

$$\begin{aligned}
> \alpha x &:= evalDG( eval( 3 q^4 dx0 - 8 q^3 r dx1 + 6 q^2 r^2 dx2 - r^4 dx3, srx ) ) : \alpha y := \\
& evalDG( eval( 3 q^4 dy0 - 8 q^3 r dy1 + 6 q^2 r^2 dy2 - r^4 dy3, srx ) ) : \\
> seq( Hook( X || i, \alpha x ), i = 1 ..3 ), seq( Hook( X || i, \alpha y ), i = 1 ..3 ), seq( Hook( Y || i, \alpha x ), i = 1 \\
& ..3 ), seq( Hook( Y || i, \alpha y ), i = 1 ..3 ) \\
& \quad 0, 0, 0, 0, 0, 0, 0, 0, 0, 0, 0, 0, 0
\end{aligned} \tag{10}$$

$$\begin{aligned}
> evalDG( \alpha x \&w ExteriorDerivative( \alpha x ) ); evalDG( \alpha y \&w ExteriorDerivative( \alpha y ) \\
& \&w ExteriorDerivative( \alpha y ) ); \\
\# simplify( evalDG( \alpha y \&w ExteriorDerivative( \alpha y ) ) ) \\
& \quad 0 dx0 \wedge dx1 \wedge dx2 \\
& \quad 0 dx0 \wedge dx1 \wedge dx2 \wedge dx3 \wedge dy0
\end{aligned} \tag{11}$$

$$\begin{aligned}
> Hook( LieDerivative( zz1, zz2 ), \alpha x ), Hook( LieDerivative( zz1, zz3 ), \alpha x ), \\
& Hook( LieDerivative( zz2, zz3 ), \alpha x ), \\
Hook( LieDerivative( zz1, zz2 ), \alpha y ), Hook( LieDerivative( zz1, zz3 ), \alpha y ), \\
& Hook( LieDerivative( zz2, zz3 ), \alpha y ) \\
& \quad 0, 0, 0, 0, 0, 0
\end{aligned} \tag{12}$$

$$\begin{aligned}
> Hook( LieDerivative( zz1, ZZ1 ), \alpha x ), Hook( LieDerivative( zz1, ZZ2 ), \alpha x ), \\
& Hook( LieDerivative( zz1, ZZ3 ), \alpha x ), Hook( LieDerivative( zz2, ZZ1 ), \alpha x ), \\
Hook( LieDerivative( zz2, ZZ2 ), \alpha x ), Hook( LieDerivative( zz2, ZZ3 ), \alpha x ), \\
& Hook( LieDerivative( zz3, ZZ1 ), \alpha x ), Hook( LieDerivative( zz3, ZZ2 ), \alpha x ), \\
Hook( LieDerivative( zz3, ZZ3 ), \alpha x ) \\
& \quad 0, 0, 0, 0, 0, 0, 0, 0, 0
\end{aligned} \tag{13}$$

$$\begin{aligned}
> simplify( eval( [ Hook( LieDerivative( zz1, ZZ1 ), \alpha y ), Hook( LieDerivative( zz1, ZZ2 ), \alpha y ), \\
& Hook( LieDerivative( zz1, ZZ3 ), \alpha y ), Hook( LieDerivative( zz2, ZZ1 ), \alpha y ), \\
Hook( LieDerivative( zz2, ZZ2 ), \alpha y ), Hook( LieDerivative( zz2, ZZ3 ), \alpha y ), \\
& Hook( LieDerivative( zz3, ZZ1 ), \alpha y ), Hook( LieDerivative( zz3, ZZ2 ), \alpha y ), \\
Hook( LieDerivative( zz3, ZZ3 ), \alpha y ) ], srx ) ) \text{ assuming } r > 0, t < 0 \\
& \quad [-12 I r^2 q^3 t, 12 I r^3 q^2 t, 0, 12 I r^3 q^2 t, -12 I r^4 q t, 0, 0, 0, 0]
\end{aligned} \tag{14}$$

$$\begin{aligned}
> k1 &:= eval( evalDG( r zz1 + q zz2 ), srx ) : k2 := zz3 : K1 := eval( evalDG( r ZZ1 + q ZZ2 ), \\
& srx ) : K2 := ZZ3 : \\
& simplify( [ seq( seq( Hook( LieDerivative( k || i, ZZ || j ), \alpha y ), i = 1 ..2 ), j = 1 ..3 ) ] ) \\
& \quad [0, 0, 0, 0, 0, 0]
\end{aligned} \tag{15}$$

$$\begin{aligned}
> \alpha 1x &:= eval( evalDG( q^2 dx0 - 2 r q dx1 + r^2 dx2 ), srx ) : \alpha 2x := eval( evalDG( 3 q^4 dx0 \\
& - 4 r q^3 dx1 + r^4 dx3 ), srx ) :
\end{aligned}$$

$$\alpha 1y := eval(evalDG(q^2 dy0 - 2 r q dy1 + r^2 dy2), srx) : \alpha 2y := eval(evalDG(3 q^4 dy0 - 4 r q^3 dy1 + r^4 dy3), srx) :$$

$$> DGsimplify(simplify(eval(evalDG(\alpha x - 6 q^2 \alpha 1x + \alpha 2x), srx)) assuming r > 0, t < 0),$$

$$DGsimplify(simplify(eval(evalDG(\alpha y - 6 q^2 \alpha 1y + \alpha 2y), srx)) assuming r > 0, t < 0)$$

$$[0 dx0, 0 dx0] \quad (16)$$

$$> \alpha 1z := evalDG(\alpha 1x + I \alpha 1y) : \alpha 2z := evalDG(\alpha 2x + I \alpha 2y) : simplify([seq(Hook(k||i, \alpha 1z), i = 1..2), seq(Hook(k||i, \alpha 2z), i = 1..2), seq(Hook(ZZ||j, \alpha 1z), j = 1..3), seq(Hook(ZZ||j, \alpha 2z), j = 1..3)])$$

$$[0, 0, 0, 0, 0, 0, 0, 0, 0, 0] \quad (17)$$

$$> simplify([seq(Hook(k||i, \alpha 1x), i = 1..2), seq(Hook(k||i, \alpha 2x), i = 1..2), seq(Hook(k||i, \alpha 1y), i = 1..2), seq(Hook(k||i, \alpha 2y), i = 1..2), seq(Hook(K||i, \alpha 1x), i = 1..2), seq(Hook(K||i, \alpha 2x), i = 1..2), seq(Hook(K||i, \alpha 1y), i = 1..2), seq(Hook(K||i, \alpha 2y), i = 1..2)])$$

$$[0, 0, 0, 0, 0, 0, 0, 0, 0, 0, 0, 0, 0, 0, 0] \quad (18)$$

$$> simplify(eval([seq(seq(Hook(LieDerivative(k||i, ZZ||j), \alpha 1z), i = 1..2), j = 1..3), seq(seq(Hook(LieDerivative(k||i, ZZ||j), \alpha 2z), i = 1..2), j = 1..3)], srx)) assuming r > 0, t < 0$$

$$[3 r^3 q t, r^3 q, -3 r^4 t, -r^4, 0, 0, 18 r^3 q^3 t, 6 r^3 q^3, -18 r^4 q^2 t, -6 r^4 q^2, 0, 0] \quad (19)$$

$$> L := evalDG(a1 k1 + a2 k2) : simplify(eval([seq(Hook(LieDerivative(L, ZZ||j), \alpha 1z), j = 1..3), seq(Hook(LieDerivative(L, ZZ||j), \alpha 2z), j = 1..3)], srx)) assuming r > 0, t < 0$$

$$[r^3 q (3 t a1 + a2), -3 a1 r^4 t - a2 r^4, 0, 6 r^3 q^3 (3 t a1 + a2), -6 r^4 q^2 (3 t a1 + a2), 0] \quad (20)$$

$$> L := evalDG(k1 - 3 t k2) : simplify(eval([seq(Hook(LieDerivative(L, ZZ||j), \alpha 1z), j = 1..3), seq(Hook(LieDerivative(L, ZZ||j), \alpha 2z), j = 1..3)], srx)) assuming r > 0, t < 0$$

$$[0, 0, 0, 0, 0, 0] \quad (21)$$

$$> \alpha 11x := eval(evalDG(q dx0 - r dx1), srx) : \alpha 12x := eval(evalDG(q^2 dx0 - r^2 dx2), srx) :$$

$$\alpha 22x := eval(evalDG(q^4 dx0 - r^4 dx3), srx) :$$

$$\alpha 11y := eval(evalDG(q dy0 - r dy1), srx) : \alpha 12y := eval(evalDG(q^2 dy0 - r^2 dy2), srx) :$$

$$\alpha 22y := eval(evalDG(q^4 dy0 - r^4 dy3), srx) :$$

$$> \alpha 11z := evalDG(\alpha 11x + I \alpha 11y) : \alpha 12z := evalDG(\alpha 12x + I \alpha 12y) : \alpha 22z := evalDG(\alpha 22x + I \alpha 22y) :$$

$$simplify(eval([Hook(L, \alpha 11z), Hook(L, \alpha 12z), Hook(L, \alpha 22z), seq(Hook(ZZ||j, \alpha 11z), j = 1..3), seq(Hook(ZZ||j, \alpha 12z), j = 1..3), seq(Hook(ZZ||j, \alpha 22z), j = 1..3)], srx)) assuming r > 0, t < 0$$

$$[0, 0, 0, 0, 0, 0, 0, 0, 0, 0, 0, 0] \quad (22)$$

$$> simplify(eval([seq(Hook(LieDerivative(L, ZZ||j), \alpha 11z), j = 1..3), seq(Hook(LieDerivative(L, ZZ||j), \alpha 12z), j = 1..3), seq(Hook(LieDerivative(L, ZZ||j), \alpha 22z), j = 1..3)], srx)) assuming r > 0, t < 0$$

$$\left[ -2 r^3 q, 2 r^4, \frac{3 r^4}{2}, -4 q^2 r^3, 4 r^4 q, 3 r^4 q, -8 r^3 q^4, 8 r^4 q^3, 6 r^4 q^3 \right] \quad (23)$$

>

Let us find symmetries of the tube over tangent to rational normal cone in R4. This is a 3-nondegenerate 7D hypersurface type CR manifold.

The equation for symmetries is equivalent to a functional equation that we resolve in steps by simplifications.

Since we work with tube domains, the equation on preservation of the x-equation only plays a role, so we simplify the vector field  $X = \text{Re}[\dots]$  and use parametric presentation of  $\text{Sigma}_3 = \{H=0\}$ .

>  $X := \text{evalDG}(\text{add}(((f \parallel i)(z_0, z_1, z_2, z_3) + (F \parallel i)(Z_0, Z_1, Z_2, Z_3)) D_x \parallel i, i = 0 \dots 3)) :$

>  $H := 16 x_1^4 x_3 - 8 x_1^2 x_2^3 - 24 x_0 x_1^2 x_2 x_3 + 9 x_0 x_2^4 + 6 x_0^2 x_2^2 x_3 + x_0^3 x_3^2 :$   
 $\text{simplify}(\text{eval}(H, \text{sxr}))$

0

(24)

>  $\text{eqn} := \text{simplify}\left(\frac{1}{16 r^8 t^3 (q + t)} \text{eval}(\text{eval}(\text{LieDerivative}(X, H), \{\text{seq}(z \parallel i = x \parallel i + I y \parallel i, i = 0 \dots 3), \text{seq}(Z \parallel i = x \parallel i - I y \parallel i, i = 0 \dots 3)\}), \text{sxr})\right)$

$\text{eqn} := -3 q^4 f_0(r^4 + I y_0, r^3 (q + t) + I y_1, q (q + 2 t) r^2 + I y_2, q^4 + 4 q^3 t + I y_3)$   
 $- 3 q^4 F_0(r^4 - I y_0, r^3 (q + t) - I y_1, q (q + 2 t) r^2 - I y_2, q^4 + 4 q^3 t - I y_3)$   
 $+ 8 q^3 f_1(r^4 + I y_0, r^3 (q + t) + I y_1, q (q + 2 t) r^2 + I y_2, q^4 + 4 q^3 t + I y_3) r$   
 $+ 8 q^3 r F_1(r^4 - I y_0, r^3 (q + t) - I y_1, q (q + 2 t) r^2 - I y_2, q^4 + 4 q^3 t - I y_3)$   
 $- 6 q^2 f_2(r^4 + I y_0, r^3 (q + t) + I y_1, q (q + 2 t) r^2 + I y_2, q^4 + 4 q^3 t + I y_3) r^2$   
 $- 6 q^2 F_2(r^4 - I y_0, r^3 (q + t) - I y_1, q (q + 2 t) r^2 - I y_2, q^4 + 4 q^3 t - I y_3) r^2 + f_3(r^4$   
 $+ I y_0, r^3 (q + t) + I y_1, q (q + 2 t) r^2 + I y_2, q^4 + 4 q^3 t + I y_3) r^4 + F_3(r^4 - I y_0, r^3 (q$   
 $+ t) - I y_1, q (q + 2 t) r^2 - I y_2, q^4 + 4 q^3 t - I y_3) r^4$

(25)

>  $\text{simplify}(\text{eval}(\text{eqn}, \{r = 0, t = 0\})); \text{simplify}(\text{eval}(\text{eqn}, \{q = 0\}))$   
 $- 3 q^4 (f_0(I y_0, I y_1, I y_2, q^4 + I y_3) + F_0(-I y_0, -I y_1, -I y_2, q^4 - I y_3))$   
 $r^4 (f_3(r^4 + I y_0, r^3 t + I y_1, I y_2, I y_3) + F_3(r^4 - I y_0, r^3 t - I y_1, -I y_2, -I y_3))$

(26)

>  $X := \text{evalDG}((f_0(z_0, z_1, z_2) - f_0(-Z_0, -Z_1, -Z_2)) D_{x_0} + \text{add}(((f \parallel i)(z_0, z_1, z_2, z_3) + (F \parallel i)(Z_0, Z_1, Z_2, Z_3)) D_x \parallel i, i = 1 \dots 2) + (f_3(z_2, z_3) - f_3(-Z_2, -Z_3)) D_{x_3}) :$

>  $\text{eqn} := \text{simplify}\left(\frac{1}{16 r^8 t^3 (q + t)} \text{eval}(\text{eval}(\text{LieDerivative}(X, H), \{\text{seq}(z \parallel i = x \parallel i + I y \parallel i, i = 0 \dots 3), \text{seq}(Z \parallel i = x \parallel i - I y \parallel i, i = 0 \dots 3)\}), \text{sxr})\right) :$

>  $\text{simplify}(\text{eval}(\text{diff}(\text{eqn}, q, t, q), \{t = 0, q = 0\})), \text{simplify}(\text{eval}(\text{diff}(\text{eqn}, r, t, r), \{t = 0, r = 0\}))$   
 $- 12 r^5 (D_2(F_2)(r^4 - I y_0, -I y_1, -I y_2, -I y_3) + D_2(f_2)(r^4 + I y_0, I y_1, I y_2, I y_3)),$   
 $- 24 q^5 (2 D_4(f_2)(I y_0, I y_1, I y_2, q^4 + I y_3) + 2 D_4(F_2)(-I y_0, -I y_1, -I y_2, q^4 - I y_3)$   
 $+ D_3(f_0)(I y_0, I y_1, I y_2))$

(27)

>  $\text{simplify}(\text{eval}(\text{diff}(\text{eqn}, r), \{r = 0\})), \text{simplify}(\text{eval}(\text{diff}(\text{eqn}, q), \{q = 0\}))$   
 $8 q^3 (f_1(I y_0, I y_1, I y_2, q^4 + 4 q^3 t + I y_3) + F_1(-I y_0, -I y_1, -I y_2, q^4 + 4 q^3 t - I y_3)),$

(28)

$$4 D_1(f_3)(Iy2, Iy3) t r^6$$

$$> X := evalDG((f_0(z_0, z_1, z_2) - f_0(-Z_0, -Z_1, -Z_2)) D_{x0} + (f_1(z_0, z_1, z_2) - f_1(-Z_0, -Z_1, -Z_2)) D_{x1} + (f_2(z_1, z_2, z_3) - f_2(-Z_1, -Z_2, -Z_3)) D_{x2} + (f_3(z_3) - f_3(-Z_3)) D_{x3}) :$$

$$> eqn := simplify\left(\frac{1}{16 r^8 t^3 (q + t)} eval(eval(LieDerivative(X, H), \{seq(z \| i = x \| i + Iy \| i, i = 0 ..3), seq(Z \| i = x \| i - Iy \| i, i = 0 ..3)\}), sxr)\right) :$$

$$> simplify(eval(diff(eqn, q, q), \{q = 0\})), simplify(eval(diff(eqn, r, r), \{r = 0\}))$$

$$12 r^2 (f_2(-r^3 t + Iy1, Iy2, Iy3) - f_2(r^3 t + Iy1, Iy2, Iy3)), -12 (-f_2(Iy1, Iy2, -q^4 - 4 q^3 t + Iy3) + f_2(Iy1, Iy2, q^4 + 4 q^3 t + Iy3) + (q^4 + 2 q^3 t) D_3(f_0)(Iy0, Iy1, Iy2)) q^2 \quad (29)$$

$$> X := evalDG((f_0(z_0, z_1) - f_0(-Z_0, -Z_1)) D_{x0} + (f_1(z_0, z_1, z_2) - f_1(-Z_0, -Z_1, -Z_2)) D_{x1} + (f_2(z_2) - f_2(-Z_2)) D_{x2} + (f_3(z_3) - f_3(-Z_3)) D_{x3}) :$$

$$> eqn := simplify\left(\frac{1}{16 r^8 t^3 (q + t)} eval(eval(LieDerivative(X, H), \{seq(z \| i = x \| i + Iy \| i, i = 0 ..3), seq(Z \| i = x \| i - Iy \| i, i = 0 ..3)\}), sxr)\right) :$$

$$> simplify(eval(diff(eqn, r, r, r), \{r = 0\})), simplify(eval(diff(eqn, q, q, q), \{q = 0\}))$$

$$-36 \left( \left( -\frac{8q}{3} - \frac{16t}{3} \right) D_3(f_1)(Iy0, Iy1, Iy2) + D_2(f_0)(Iy0, Iy1) (q + t) \right) q^4, \quad (30)$$

$$48 r (D(f_3)(Iy3) r^3 t - 3 D(f_2)(Iy2) r^3 t + f_1(r^4 + Iy0, r^3 t + Iy1, Iy2) - f_1(-r^4 + Iy0, -r^3 t + Iy1, Iy2))$$

$$> X := evalDG((f_0(z_0) - f_0(-Z_0)) D_{x0} + (f_1(z_1) - f_1(-Z_1)) D_{x1} + (f_2(z_2) - f_2(-Z_2)) D_{x2} + f_3 \cdot (z_3 + Z_3) D_{x3}) :$$

$$> eqn := simplify\left(\frac{1}{16 r^8 t^3 (q + t)} eval(eval(LieDerivative(X, H), \{seq(z \| i = x \| i + Iy \| i, i = 0 ..3), seq(Z \| i = x \| i - Iy \| i, i = 0 ..3)\}), sxr)\right) :$$

$$> simplify(eval(diff(eqn, r, r, r), \{r = 0\})), simplify(eval(diff(eqn, q, q, q), \{q = 0\}))$$

$$0, 48 r (f_3 r^3 t - 3 D(f_2)(Iy2) r^3 t - f_1(-r^3 t + Iy1) + f_1(r^3 t + Iy1)) \quad (31)$$

$$> X := evalDG((f_0(z_0) - f_0(-Z_0)) D_{x0} + f_1 \cdot (z_1 + Z_1) D_{x1} + f_2 \cdot (z_2 + Z_2) D_{x2} + (3 f_2 - 2 f_1) \cdot (z_3 + Z_3) D_{x3}) :$$

$$> eqn := simplify\left(\frac{1}{16 r^8 t^3 (q + t)} eval(eval(LieDerivative(X, H), \{seq(z \| i = x \| i + Iy \| i, i = 0 ..3), seq(Z \| i = x \| i - Iy \| i, i = 0 ..3)\}), sxr)\right) :$$

$$> simplify(eval(diff(eqn, r, r, r, r), \{r = 0\})), simplify(eval(diff(eqn, q, q, q, q), \{q = 0\}))$$

$$-144 (-2 f_1 + f_2 + D(f_0)(Iy0)) q^4, 72 f_0(-r^4 + Iy0) - 72 f_0(r^4 + Iy0) + (288 f_1 \quad (32)$$

$$-144 f_2) r^4$$

```

> X := evalDG((2 f1 - f2) · (z0 + Z0) D_x0 + f1 · (z1 + Z1) D_x1 + f2 · (z2 + Z2) D_x2
+ (3 f2 - 2 f1) · (z3 + Z3) D_x3) :
> eqn := simplify( (1 / (16 r^8 t^3 (q + t)) eval(eval(LieDerivative(X, H), {seq(z || i = x || i + I y || i, i = 0
..3), seq(Z || i = x || i - I y || i, i = 0 ..3)}), sxr) ) :
> eqn
0

```

(33)

Thus the symmetry is linear in R4(x): it is 2-dimensional algebra of scalings. Plus 4 shifts along y-directions in R4(y). Altogether 6.

```

> z0 D_z0 + z1 D_z1 + z2 D_z2 + z3 D_z3 + Z0 D_Z0 + Z1 D_Z1 + Z2 D_Z2 + Z3 D_Z3,
2 z0 D_z0 + z1 D_z1 - 2 z3 D_z3 + 2 Z0 D_Z0 + Z1 D_Z1 - 2 Z3 D_Z3,
I/2 · (D_z0 - D_Z0), I/2 · (D_z1 - D_Z1), I/2 · (D_z2 - D_Z2), I/2 · (D_z3 - D_Z3)

```

Conclusion is the same: the symmetry is the semi-direct sum of the linear algebra a(2)<gl(4,R) and the space of translations R4(y).

For the tangent to a cone over a general curve in P3, consider a tube, and let us compute CR symmetries. Since translation along R4(y) form the maximal abelian ideal of the symmetry algebra (by what was already established) the symmetry quotients to a transformation of Σ3 in R4(x) depending on parametrization via (p,q,r). We work here in parametric form of the tube (opposite to implicit form as one constraint on x) and hence represent the symmetry X as both a holomorphic field in C4 and as a vector field on M7 projecting along R4(y) to Σ3(p,q,r).

```

> DGsetup([x0, x1, x2, x3, p, q], M) :
> X := evalDG(add(add((a || i || j) · (x || i) D_x || j, i = 0 ..3), j = 0 ..3) + (b11 p + b12 q) · D_p
+ (b21 p + b22 q) · D_q) : sxr := {x0 = p^3, x1 = p^2 q, x2 = p q^2, x3 = q^3} :
sys := eval({LieDerivative(X, x0 - p^3), LieDerivative(X, x1 - p^2 q), LieDerivative(X, x2
- p q^2), LieDerivative(X, x3 - q^3)}, sxr) :
sll := solve({seq(coeffs(expand(sys[i]), {p, q}), i = 1 ..4)}): X := DGsimplify(eval(X, sll)) :
eval(Matrix([[a00, a01, a02, a03], [a10, a11, a12, a13], [a20, a21, a22, a23], [a30, a31, a32,
a33]]), sll)

```

$$\begin{bmatrix} 3 b_{11} & b_{21} & 0 & 0 \\ 3 b_{12} & 2 b_{11} + b_{22} & 2 b_{21} & 0 \\ 0 & 2 b_{12} & b_{11} + 2 b_{22} & 3 b_{21} \\ 0 & 0 & b_{12} & 3 b_{22} \end{bmatrix}$$

(34)

```

> X := evalDG(add(add((a || i || j) · (x || i) D_x || j, i = 0 ..3), j = 0 ..3) + (b11 p + b12 q) · D_p
+ (b21 p + b22 q) · D_q) : sxr := {x0 = p^4, x1 = p^3 q, x2 = p^2 q^2 + p q^3, x3 = q^4} :
sys := eval({LieDerivative(X, x0 - p^4), LieDerivative(X, x1 - p^3 q), LieDerivative(X, x2
- p^2 q^2 - p q^3), LieDerivative(X, x3 - q^4)}, sxr) :
sll := solve({seq(coeffs(expand(sys[i]), {p, q}), i = 1 ..4)}): X := DGsimplify(eval(X, sll)) :

```

$eval(Matrix([ [a00, a01, a02, a03], [a10, a11, a12, a13], [a20, a21, a22, a23], [a30, a31, a32, a33] ]), sll)$

$$\begin{bmatrix} 4b_{22} & 0 & 0 & 0 \\ 0 & 4b_{22} & 0 & 0 \\ 0 & 0 & 4b_{22} & 0 \\ 0 & 0 & 0 & 4b_{22} \end{bmatrix} \quad (35)$$

>  $DGsetup([x0, x1, x2, x3, p, q, r], M) :$   
>  $X := evalDG(add(add((a||i||j) \cdot (x||i) D_x||j, i=0..3), j=0..3) + (b11p + b12q + b13r) \cdot D_p + (b21p + b22q + b23r) \cdot D_q + (b31p + b32q + b33r) \cdot D_r) :$   
 $sxr := \{x0 = p^4 + 4p^3r, x1 = p^3q + 3p^2qr, x2 = p^2q^2 + pq^3 + 2pq^2r + q^3r, x3 = q^4\} :$   
 $sys := eval(\{LieDerivative(X, x0 - (p^4 + 4p^3r)), LieDerivative(X, x1 - (p^3q + 3p^2qr)), LieDerivative(X, x2 - (p^2q^2 + pq^3 + 2pq^2r + q^3r)), LieDerivative(X, x3 - q^4)\}, sxr) :$   
 $sll := solve(\{seq(coeffs(expand(sys[i]), \{p, q, r\}), i=1..4)\} : X := DGsimplify(eval(X, sll)) :$   
 $eval(Matrix([ [a00, a01, a02, a03], [a10, a11, a12, a13], [a20, a21, a22, a23], [a30, a31, a32, a33] ]), sll)$

$$\begin{bmatrix} 4b_{22} & 0 & 0 & 0 \\ 0 & 4b_{22} & 0 & 0 \\ 0 & 0 & 4b_{22} & 0 \\ 0 & 0 & 0 & 4b_{22} \end{bmatrix} \quad (36)$$

Above we computed affine symmetries in parametric representation of a hypersurface, below we address CR-symmetries

>  $DGsetup([x0, x1, x2, x3, y0, y1, y2, y3, p, q, r], R8) :$   
>  $X := evalDG(add((f||i)(z0, z1, z2, z3) + (F||i)(Z0, Z1, Z2, Z3)) D_x||i, i=0..3) + g1(p, q, r) D_p + g2(p, q, r) D_q + g3(p, q, r) D_r) :$   
>  $sxr := \{x0 = p^4 + 4p^3r, x1 = p^3q + 3p^2qr, x2 = p^2q^2 + pq^3 + 2pq^2r + q^3r, x3 = q^4\} :$   
 $eqq := \{seq(lhs(sxr[i]) - rhs(sxr[i]), i=1..4)\} :$   
>  $eqn := simplify([seq(eval(eval(LieDerivative(X, eqq[j])), \{seq(z||i=x||i + Iy||i, i=0..3), seq(Z||i=x||i - Iy||i, i=0..3)\}), sxr), j=1..4)])$   
 $eqn := [f3(p^4 + 4p^3r + Iy0, p^2(p + 3r)q + Iy1, (p + r)q^3 + p(p + 2r)q^2 + Iy2, q^4 + Iy3) + F3(p^4 + 4p^3r - Iy0, p^2(p + 3r)q - Iy1, (p + r)q^3 + p(p + 2r)q^2 - Iy2, q^4 - Iy3) - 4g2(p, q, r)q^3, -4g1(p, q, r)p^3 - 12g1(p, q, r)p^2r - 4g3(p, q, r)p^3 + f0(p^4 + 4p^3r + Iy0, p^2(p + 3r)q + Iy1, (p + r)q^3 + p(p + 2r)q^2 + Iy2, q^4 + Iy3) + F0(p^4 + 4p^3r - Iy0, p^2(p + 3r)q - Iy1, (p + r)q^3 + p(p + 2r)q^2 - Iy2, q^4 - Iy3), -3g1(p, q, r)p^2q - 6g1(p, q, r)pqr - 3g3(p, q, r)p^2q - g2(p, q, r)p^3 - 3g2(p, q, r)p^2r + f1(p^4 + 4p^3r + Iy0, p^2(p + 3r)q + Iy1, (p + r)q^3 + p(p + 2r)q^2 + Iy2, q^4 + Iy3) + F1(p^4 + 4p^3r - Iy0, p^2(p + 3r)q - Iy1, (p + r)q^3 + p(p + 2r)q^2 - Iy2, q^4 - Iy3)] \quad (37)$

$$+ r) q^3 + p (p + 2 r) q^2 - I y_2, q^4 - I y_3), F2(p^4 + 4 p^3 r - I y_0, p^2 (p + 3 r) q - I y_1, (p + r) q^3 + p (p + 2 r) q^2 - I y_2, q^4 - I y_3) + f2(p^4 + 4 p^3 r + I y_0, p^2 (p + 3 r) q + I y_1, (p + r) q^3 + p (p + 2 r) q^2 + I y_2, q^4 + I y_3) + ((-3 p - 3 r) q^2 + (-2 p^2 - 4 p r) q) g2(p, q, r) + (-q^3 + (-2 p - 2 r) q^2) g1(p, q, r) + g3(p, q, r) (-2 p q^2 - q^3)]$$

$$\begin{aligned} &> eval(eqn[1], q = 0); eval(eqn[2], p = 0); eval(eqn[3], p = 0); eval(eqn[4], q = 0) \\ &\quad f3(p^4 + 4 p^3 r + I y_0, I y_1, I y_2, I y_3) + F3(p^4 + 4 p^3 r - I y_0, -I y_1, -I y_2, -I y_3) \\ &\quad f0(I y_0, I y_1, q^3 r + I y_2, q^4 + I y_3) + F0(-I y_0, -I y_1, q^3 r - I y_2, q^4 - I y_3) \\ &\quad f1(I y_0, I y_1, q^3 r + I y_2, q^4 + I y_3) + F1(-I y_0, -I y_1, q^3 r - I y_2, q^4 - I y_3) \\ &\quad F2(p^4 + 4 p^3 r - I y_0, -I y_1, -I y_2, -I y_3) + f2(p^4 + 4 p^3 r + I y_0, I y_1, I y_2, I y_3) \end{aligned} \quad (38)$$

$$\begin{aligned} &> X := evalDG((f0(z0, z1) - f0(-Z0, -Z1)) D_x0 + (f1(z0, z1) - f1(-Z0, -Z1)) D_x1 \\ &\quad + (f2(z1, z2, z3) - f2(-Z1, -Z2, -Z3)) D_x2 + (f3(z1, z2, z3) - f3(-Z1, -Z2, \\ &\quad -Z3)) D_x3 + g1(p, q, r) D_p + g2(p, q, r) D_q + g3(p, q, r) D_r) : \end{aligned}$$

$$\begin{aligned} &> eqn := simplify([seq(eval(LieDerivative(X, eqq[j])), {seq(z || i = x || i + I y || i, i = 0 .. 3), \\ &\quad seq(Z || i = x || i - I y || i, i = 0 .. 3)}), sxx), j = 1 .. 4)]) : \end{aligned}$$

$$\begin{aligned} &> eval(diff(eqn[1], q), {q = 0}); eval(diff(eqn[1], q, q), {q = 0}); eval(diff(eqn[1], q, q, q, q), \\ &\quad {p = 0, q = 0, r = 0}); \\ &\quad factor(eval(diff(eqn[2], p, p), {p = 0})); factor(eval(diff(eqn[2], p, p, p, p), {p = 0, q = 0, r \\ &\quad = 0})); \\ &\quad eval(diff(eqn[3], p, p, q, r), {p = 0, q = 0, r = 0}); eval(diff(eqn[3], p, p, p, r), {p = 0, q = 0, r \\ &\quad = 0}); eval(diff(eqn[3], p), {p = 0}); \\ &\quad eval(diff(eqn[4], p, p, q, r), {p = 0, q = 0, r = 0}); eval(diff(eqn[4], q, q, q, r), {p = 0, q = 0, r \\ &\quad = 0}); eval(diff(eqn[4], q, q, q, q), {p = 0, q = 0, r = 0}) \end{aligned}$$

$$\begin{aligned} &\quad 2 D_1(f3)(I y_1, I y_2, I y_3) p^2 (p + 3 r) \\ &\quad 4 D_2(f3)(I y_1, I y_2, I y_3) p (p + 2 r) \\ &\quad 48 D_3(f3)(I y_1, I y_2, I y_3) - 96 D_2(g2)(0, 0, 0) \\ &\quad - 12 r (-D_2(f0)(I y_0, I y_1) q + 2 g1(0, q, r)) \\ &\quad - 96 D_1(g1)(0, 0, 0) - 96 D_1(g3)(0, 0, 0) + 48 D_1(f0)(I y_0, I y_1) \\ &- 12 D_1(g1)(0, 0, 0) - 6 D_3(g1)(0, 0, 0) + 12 D_2(f1)(I y_0, I y_1) - 6 D_3(g3)(0, 0, 0) \\ &\quad - 6 D_2(g2)(0, 0, 0) \\ &\quad - 18 D_1(g2)(0, 0, 0) - 6 D_3(g2)(0, 0, 0) + 48 D_1(f1)(I y_0, I y_1) \\ &\quad - 6 g1(0, q, r) q r \\ &\quad 12 D_1(f2)(I y_1, I y_2, I y_3) - 4 D_3(g2)(0, 0, 0) - 8 D_1(g2)(0, 0, 0) \\ &- 6 D_3(g3)(0, 0, 0) - 12 D_2(g1)(0, 0, 0) - 18 D_2(g2)(0, 0, 0) + 12 D_2(f2)(I y_1, I y_2, I y_3) \\ &\quad - 6 D_3(g1)(0, 0, 0) \\ &\quad - 24 D_2(g3)(0, 0, 0) - 24 D_2(g1)(0, 0, 0) + 48 D_3(f2)(I y_1, I y_2, I y_3) \end{aligned} \quad (39)$$

Already here we observe that the symmetry is affine in R4(x) so the conclusion follows, but let us finish it in CR methods

$$\begin{aligned}
& \triangleright X := evalDG((c1 z0 + c2 z1 + C1 Z0 + C2 Z1) D_x0 + (c3 z0 + c4 z1 + C3 Z0 \\
& \quad + C4 Z1) D_x1 + (c5 z1 + c6 z2 + c7 z3 + C5 Z1 + C6 Z2 + C7 Z3) D_x2 + (c8 z3 \\
& \quad + C8 Z3) D_x3 + g1(p, q, r) p D_p + g2(p, q, r) q D_q + g3(p, q, r) D_r) : \\
& \triangleright eqn := simplify([seq(eval(eval(LieDerivative(X, eqq[j])), {seq(z||i=x||i+Iy||i, i=0..3), \\
& \quad seq(Z||i=x||i-Iy||i, i=0..3)}), sxx), j=1..4)]) : \\
& \triangleright eqn[1]; eqn[2]; eqn[3]; eqn[4] \\
& \quad -4 g2(p, q, r) q^4 + (C8 + c8) q^4 - I y3 (C8 - c8) \\
& -4 p^3 (p + 3 r) g1(p, q, r) - 4 g3(p, q, r) p^3 + (C1 + c1) p^4 + ((4 C1 + 4 c1) r + q (C2 \\
& \quad + c2)) p^3 + 3 q r (C2 + c2) p^2 - I C1 y0 - I C2 y1 + I c1 y0 + I c2 y1 \\
& -3 p^2 q (p + 2 r) g1(p, q, r) - p^2 q (p + 3 r) g2(p, q, r) - 3 g3(p, q, r) p^2 q + (C3 \\
& \quad + c3) p^4 + (q (C4 + c4) + 4 r (C3 + c3)) p^3 + 3 q r (C4 + c4) p^2 - I C3 y0 - I C4 y1 \\
& \quad + I c3 y0 + I c4 y1 \\
& -2 \left( \left( \frac{3p}{2} + \frac{3r}{2} \right) q + p (p + 2 r) \right) q^2 g2(p, q, r) - 2 p q^2 \left( p + \frac{q}{2} + r \right) g1(p, q, r) \quad (40) \\
& \quad + g3(p, q, r) (-2 p q^2 - q^3) + (C7 + c7) q^4 + (C6 + c6) (p + r) q^3 + p (C6 \\
& \quad + c6) (p + 2 r) q^2 + p^2 (C5 + c5) (p + 3 r) q - I C6 y2 + I c6 y2 - I C5 y1 + I c5 y1 \\
& \quad - I (C7 - c7) y3
\end{aligned}$$

$$\begin{aligned}
& \triangleright X := evalDG((c1 \cdot (z0 + Z0) + c2 \cdot (z1 + Z1)) D_x0 + (c3 \cdot (z0 + Z0) + c4 \cdot (z1 \\
& \quad + Z1)) D_x1 + (c5 \cdot (z1 + Z1) + c6 \cdot (z2 + Z2) + c7 \cdot (z3 + Z3)) D_x2 + c8 \cdot (z3 \\
& \quad + Z3) D_x3 + g1(p, q, r) p D_p + \frac{1}{2} c8 q D_q + g3(p, q, r) D_r) : \\
& \triangleright eqn := simplify([seq(eval(eval(LieDerivative(X, eqq[j])), {seq(z||i=x||i+Iy||i, i=0..3), \\
& \quad seq(Z||i=x||i-Iy||i, i=0..3)}), sxx), j=1..4)]) : \\
& \triangleright eqn[1]; simplify(eqn[2]); simplify(eqn[3]); simplify(eqn[4]) \\
& \quad 0 \\
& \quad 2 p^2 (-2 p (p + 3 r) g1(p, q, r) - 2 g3(p, q, r) p + c1 p^2 + (4 c1 r + c2 q) p + 3 c2 q r) \\
& \quad 2 \left( -\frac{3 q (p + 2 r) g1(p, q, r)}{2} - \frac{3 g3(p, q, r) q}{2} + (p + 3 r) \left( c4 - \frac{c8}{4} \right) q + p c3 (p \right. \\
& \quad \left. + 4 r) \right) p^2 \\
& \quad 2 \left( -p \left( p + \frac{q}{2} + r \right) q g1(p, q, r) - \left( p + \frac{q}{2} \right) q g3(p, q, r) + c7 q^3 + \left( c6 - \frac{3 c8}{4} \right) (p \right. \quad (41) \\
& \quad \left. + r) q^2 + (p + 2 r) p \left( c6 - \frac{c8}{2} \right) q + c5 p^2 (p + 3 r) \right) q
\end{aligned}$$

$$\triangleright solve\left(\left\{coeffs\left(eliminate\left(\left\{(-2 p (p + 3 r) g1 - 2 g3 p + c1 p^2 + (4 c1 r + c2 q) p\right.\right.\right.\right.
\right.$$

$$\begin{aligned}
& + 3 c_2 q r), \left( -\frac{3 q (p + 2 r) g_1}{2} - \frac{3 g_3 q}{2} + (p + 3 r) \left( c_4 - \frac{c_8}{4} \right) q + p c_3 (p \right. \\
& + 4 r) \left. \right), \left( -p \left( p + \frac{q}{2} + r \right) q g_1 - \left( p + \frac{q}{2} \right) q g_3 + c_7 q^3 + \left( c_6 - \frac{3 c_8}{4} \right) (p \right. \\
& + r) q^2 + (p + 2 r) p \left( c_6 - \frac{c_8}{2} \right) q + c_5 p^2 (p + 3 r) \left. \right) \left. \right\}, \{g_1, g_3\} \left. \right) [2][1], \{p, q, r\} \left. \right) \left. \right\} \\
& \left. \right) \\
& \{c_1 = c_8, c_2 = 0, c_3 = 0, c_4 = c_8, c_5 = 0, c_6 = c_8, c_7 = 0, c_8 = c_8\} \tag{42}
\end{aligned}$$

$$\begin{aligned}
& \text{> } X := \text{evalDG} \left( (z_0 + Z_0) D_{x0} + (z_1 + Z_1) D_{x1} + (z_2 + Z_2) D_{x2} + (z_3 + Z_3) D_{x3} \right. \\
& \quad \left. + g_1(p, q, r) p D_p + \frac{1}{2} q D_q + g_3(p, q, r) D_r \right) : \\
& \text{> } \text{eqn} := \text{simplify} \left( [\text{seq}(\text{eval}(\text{eval}(\text{LieDerivative}(X, \text{eqq}[j])), \{ \text{seq}(z \parallel i = x \parallel i + I y \parallel i, i = 0 \dots 3), \right. \\
& \quad \left. \text{seq}(Z \parallel i = x \parallel i - I y \parallel i, i = 0 \dots 3) \}), \text{sxr}), j = 1 \dots 4) ] \right) : \\
& \text{> } \text{eqn}[1]; \text{simplify}(\text{eqn}[2]); \text{simplify}(\text{eqn}[3]); \text{simplify}(\text{eqn}[4]) \\
& \quad 0 \\
& \quad -4 \left( (p + 3 r) g_1(p, q, r) - \frac{p}{2} - 2 r + g_3(p, q, r) \right) p^3 \\
& \quad -3 p^2 \left( (p + 2 r) g_1(p, q, r) - \frac{p}{2} - \frac{3 r}{2} + g_3(p, q, r) \right) q \\
& -2 \left( \left( p + \frac{q}{2} + r \right) p g_1(p, q, r) + \left( p + \frac{q}{2} \right) g_3(p, q, r) - \frac{p^2}{2} + \left( -\frac{q}{4} - r \right) p \right. \\
& \quad \left. - \frac{q r}{4} \right) q^2 \tag{43} \\
& \text{> } \text{solve} \left( \left\{ \left( (p + 3 r) g_1 - \frac{p}{2} - 2 r + g_3 \right), \left( (p + 2 r) g_1 - \frac{p}{2} - \frac{3 r}{2} + g_3 \right), \left( \left( p + \frac{q}{2} \right. \right. \right. \\
& \quad \left. \left. + r \right) p g_1 + \left( p + \frac{q}{2} \right) g_3 - \frac{p^2}{2} + \left( -\frac{q}{4} - r \right) p - \frac{q r}{4} \right\}, \{g_1, g_3\} \right) \\
& \quad \left\{ g_1 = \frac{1}{2}, g_3 = \frac{r}{2} \right\} \tag{44}
\end{aligned}$$

$$\begin{aligned}
& \text{> } X := \text{evalDG} \left( (z_0 + Z_0) D_{x0} + (z_1 + Z_1) D_{x1} + (z_2 + Z_2) D_{x2} + (z_3 + Z_3) D_{x3} \right. \\
& \quad \left. + \frac{p}{2} D_p + \frac{q}{2} D_q + \frac{r}{2} D_r \right) : \\
& \text{> } \text{eqn} := \text{simplify} \left( [\text{seq}(\text{eval}(\text{eval}(\text{LieDerivative}(X, \text{eqq}[j])), \{ \text{seq}(z \parallel i = x \parallel i + I y \parallel i, i = 0 \dots 3), \right. \\
& \quad \left. \text{seq}(Z \parallel i = x \parallel i - I y \parallel i, i = 0 \dots 3) \}), \text{sxr}), j = 1 \dots 4) ] \right) \\
& \quad \text{eqn} := [0, 0, 0, 0] \tag{45}
\end{aligned}$$

Thus we conclude that there is only one symmetry beyond the translations in y-direction, so the model has 5D symmetry.

>

Finally consider a general ruled surface  $\gamma(t)+s\gamma'(t)+t\gamma''(t)$  with no affine symmetry. The first attempt has a scaling symmetry, while the second has nothing.

> #` `[ $r^4 + 4 r^3 s + 12 r^2 t, r^3 + 3 r^2 s + 6 r t, r^2 + 2 r s + 2 t, r + s$ ]

> DGsetup([ $x0, x1, x2, x3, r, s, t$ ], M) :

> X := evalDG(add(add((a||i||j)·(x||i) D\_x||j, i = 0..3), j = 0..3) + b1·D\_r + b2·D\_s + b3·D\_t) :

sxr := { $x0 = r^4 + 4 r^3 s + 12 r^2 t, x1 = r^3 + 3 r^2 s + 6 r t, x2 = r^2 + 2 r s + 2 t, x3 = r + s$ } :

sys := eval({LieDerivative(X,  $x0 - (r^4 + 4 r^3 s + 12 r^2 t)$ ), LieDerivative(X,  $x1 - (r^3 + 3 r^2 s + 6 r t)$ ), LieDerivative(X,  $x2 - (r^2 + 2 r s + 2 t)$ ), LieDerivative(X,  $x3 - (r + s)$ )}, sxr)

sys := { $a03 (r^4 + 4 r^3 s + 12 r^2 t) + a13 (r^3 + 3 r^2 s + 6 r t) + a23 (r^2 + 2 r s + 2 t) + a33 (r + s) - b1 - b2, a00 (r^4 + 4 r^3 s + 12 r^2 t) + a10 (r^3 + 3 r^2 s + 6 r t) + a20 (r^2 + 2 r s + 2 t) + a30 (r + s) + b1 (-4 r^3 - 12 r^2 s - 24 r t) - 4 b2 r^3 - 12 b3 r^2, a01 (r^4 + 4 r^3 s + 12 r^2 t) + a11 (r^3 + 3 r^2 s + 6 r t) + a21 (r^2 + 2 r s + 2 t) + a31 (r + s) + b1 (-3 r^2 - 6 r s - 6 t) - 3 b2 r^2 - 6 b3 r, a02 (r^4 + 4 r^3 s + 12 r^2 t) + a12 (r^3 + 3 r^2 s + 6 r t) + a22 (r^2 + 2 r s + 2 t) + a32 (r + s) + b1 (-2 r - 2 s) - 2 b2 r - 2 b3$ } (46)

> tm := eliminate(% , {b1, b2, b3}) :

> sll := solve({coeffs(tm[2][1], {r, s, t})})

sll := { $a00 = 4 a33, a01 = 0, a02 = 0, a03 = 0, a10 = 0, a11 = 3 a33, a12 = 0, a13 = 0, a20 = 0, a21 = 0, a22 = 2 a33, a23 = 0, a30 = 0, a31 = 0, a32 = 0, a33 = a33$ } (47)

> sl2 := eval(tm, sll) : sll := sll union sl2[1]

sll := { $a00 = 4 a33, a01 = 0, a02 = 0, a03 = 0, a10 = 0, a11 = 3 a33, a12 = 0, a13 = 0, a20 = 0, a21 = 0, a22 = 2 a33, a23 = 0, a30 = 0, a31 = 0, a32 = 0, a33 = a33, b1 = a33 r, b2 = a33 s, b3 = 2 a33 t$ } (48)

> eval(eval(X, sll), {a33 = 1})

$4 x0 D_x0 + 3 x1 D_x1 + 2 x2 D_x2 + x3 D_x3 + r D_r + s D_s + 2 t D_t$  (49)

> #` `[ $r^4 + 4 r^3 s + 12 r^2 t, r^3 + 1 + 3 r^2 s + 6 r t, r^2 + 2 r s + 2 t, r + s$ ]

> X := evalDG(add(add((a||i||j)·(x||i) D\_x||j, i = 0..3), j = 0..3) + b1·D\_r + b2·D\_s + b3·D\_t) :

sxr := { $x0 = r^4 + 4 r^3 s + 12 r^2 t, x1 = r^3 + 1 + 3 r^2 s + 6 r t, x2 = r^2 + 2 r s + 2 t, x3 = r + s$ } :

sys := eval({LieDerivative(X,  $x0 - (r^4 + 4 r^3 s + 12 r^2 t)$ ), LieDerivative(X,  $x1 - (r^3 + 1 + 3 r^2 s + 6 r t)$ ), LieDerivative(X,  $x2 - (r^2 + 2 r s + 2 t)$ ), LieDerivative(X,  $x3 - (r + s)$ )}, sxr)

sys := { $a03 (r^4 + 4 r^3 s + 12 r^2 t) + a13 (r^3 + 3 r^2 s + 6 r t + 1) + a23 (r^2 + 2 r s + 2 t) + a33 (r + s) - b1 - b2, a00 (r^4 + 4 r^3 s + 12 r^2 t) + a10 (r^3 + 3 r^2 s + 6 r t + 1)$  (50)

$$\begin{aligned}
& + a_{20} (r^2 + 2rs + 2t) + a_{30} (r + s) + b_1 (-4r^3 - 12r^2s - 24rt) - 4b_2r^3 \\
& - 12b_3r^2, a_{01} (r^4 + 4r^3s + 12r^2t) + a_{11} (r^3 + 3r^2s + 6rt + 1) + a_{21} (r^2 + 2rs \\
& + 2t) + a_{31} (r + s) + b_1 (-3r^2 - 6rs - 6t) - 3b_2r^2 - 6b_3r, a_{02} (r^4 + 4r^3s \\
& + 12r^2t) + a_{12} (r^3 + 3r^2s + 6rt + 1) + a_{22} (r^2 + 2rs + 2t) + a_{32} (r + s) + b_1 (- \\
& - 2r - 2s) - 2b_2r - 2b_3\}
\end{aligned}$$

```

> tm := eliminate(% , {b1, b2, b3}) :
> sll := solve( {coeffs(tm[2][1], {r, s, t})} ) :
> sl2 := eval(tm, sll) : sll := sll union sl2[1] :
> DGsimplify(eval(X, sll))

```

$$0 D_{x0}$$

(51)

Finally Now we form 7D tube domain over this 3D surface, and compute its CR symmetries. As expected only translations along R4(y) are such symmetries

```

> X := evalDG(add(add((a||i||j)·(x||i) D_x||j, i=0..3), j=0..3) + b1·D_r + b2·D_s + b3
·D_t) :
sxr := {x0 = r^4 + 4r^3s + 12r^2t, x1 = r^3 + 1 + 3r^2s + 6rt, x2 = r^2 + 2rs + 2t, x3 = r
+ s} :
sys := eval( {LieDerivative(X, x0 - (r^4 + 4r^3s + 12r^2t)), LieDerivative(X, x1 - (r^3 + 1
+ 3r^2s + 6rt)), LieDerivative(X, x2 - (r^2 + 2rs + 2t)), LieDerivative(X, x3 - (r
+ s)) }, sxr) : tm := eliminate(% , {b1, b2, b3}) : sll := solve( {coeffs(tm[2][1], {r, s,
t})} ) : sl2 := eval(tm, sll) : sll := sll union sl2[1] : X := DGsimplify(eval(X, sll)) :
eval(Matrix([ [a00, a01, a02, a03], [a10, a11, a12, a13], [a20, a21, a22, a23], [a30, a31, a32,
a33]]), sll)

```

$$\begin{bmatrix} 0 & 0 & 0 & 0 \\ 0 & 0 & 0 & 0 \\ 0 & 0 & 0 & 0 \\ 0 & 0 & 0 & 0 \end{bmatrix}$$

(52)

Thus we realize symmetry dimensions 6,5,4 for 3ndg CR manifolds of hypersurface type in 7D

>
